# Supplementary material for: Optimal Covariate Weighting Increases Discoveries in High-throughput Biology
Source: arXiv:2203.05926 source file (2022-03-11)
Supplement: Supplementary file 1 [file Supplementary_material.pdf]

# Supplementary Information

## Table of Contents


1. Introduction ........ 3

2. Methods ........ 3

3. Estimating the distribution of power across tests ........ 3

**3.1. Estimating the distribution of power.** ........ 3

**3.2. Efron method for estimating power** ........ 6

4. Simulation Procedures ........ 9

**4.1 Group effect (Figure 2 and Figure 3).** ........ 9

**4.2 Ranks probability (Figure 4).** ........ 9

**4.3. Ranks probability and weight (Figure 5).** ........ 9

**4.4. Power (Figures 6 and 7).** ........ 9

5. Work Flow ........ 10

6. Additional proofs ........ 12

7. Ranks probability of test given effect size, $Pri = k\tau i$. ........ 14

**7.1. $Pri = k\tau i$ given continuous effect.** ........ 15

**7.2. $Pri = k\tau i$ given binary effect.** ........ 20

8. Probability of ranks and weights ........ 27

9. Family-wise error rate (FWER). ........ 32

**9.1. FWER when all tests are from true null models.** ........ 32

**9.2. FWER for different effect sizes.** ........ 33

**9.2.1. Continuous effects.** ........ 33

**9.2.2. Binary effects.** ........ 34

10. False discovery rate (FDR). ........ 35

**10.1. Continuous effects.** ........ 35

**10.2. Binary effects.** ........ 36

11. Power vs. effect size ........ 37

**11.1. Continuous effects.** ........ 37

**11.2. Binary effects.** ........ 37

12. Power vs. variance of test effect ........ 39

13. Power vs. proportion of true null hypothesis. ........ 41

14. Power vs. test correlation. ........ 43

15. Relationship between covariate effect and test effect........................................................................45
16. Nonlinear Relationship Between Test Effect and Covariate Effect.....................................................47
17. Data Examples.........................................................................................................................50
18. Approximate vs. exact weights. .............................................................................................53
19. Algorithm to compute CRW weights ......................................................................................54
References ....................................................................................................................................56

## 1. Introduction

In this supplementary document, additional proofs, examples, simulation figures are included to elaborate on the claims that we made in the original articles. In the following sections, we will treat the covariates similarly as the test statistics without loss of information.

## 2. Methods

In Theorem 2, we showed the mathematical derivation of the ranks probability given continuous effect $P(r_i|\tau_i)$, which is composed of two CDF $F_0$ and $F_1$. Here, we show an example of how to obtain $F_0$ and $F_1$.

**Example.** Suppose test statistic $X_j \sim N(\tau_j = 0, 1)$ under the null model. Then $P(X_j > t) = 1 - F_0(t,\ \tau = 0) = 1 - \Phi(t) = \Phi(-t)$. Under the alternative model, $P(Y_l > t) = 1 - \int F_1(t,\ \tau_l) f(\tau_l) d\tau_l = 1 - \int \Phi(t - \tau_l) f(\tau_l) d\tau_l$, where $f(\tau_l)$ is the probability density function of $\tau_l$. Sometimes an explicit result of the integral is attainable. For example, if we assume that the effect sizes follow a uniform distribution such that $\tau_l \sim U(a, b)$, then we have $P(Y_l > t) = \frac{1}{b-a}[(b-t)\Phi(b-t) - (a-t)\Phi(a-t) + \phi(b-t) - \phi(a-t)]$. Similarly, if the effect sizes follow an exponential distribution with rate parameter $\lambda$, then $P(Y_l > t) = \Phi(-t) + e^{-\lambda t} e^{\frac{\lambda^2}{2}} \Phi(t - \lambda)$. For the details see the Additional proof Section 6 of SI. Consequently, the probability of the rank of the tests given the effect size $P(r_i = k|\tau_i)$ is obtained by plugging $F_0$ and $F_1$ in Theorem 2.

We also developed a method of weight for binary effect sizes and proposed the corresponding ranks probability given the binary effects, $P(r_i|\tau)$. Computing the ranks probability given the effect, $P(r_i|\tau)$, for the binary case is similar to the computation for the continuous case. Under the null model, the effect size is 0, which is not different from the previous section. Under the alternative model, the effect size is a constant; unlike the effect size in the continuous case. Therefore, the probability of success $P(Y_l > t) = 1 - F_1(t, \tau)$ depends on the common effect size $\tau$.

**Example.** The example presented in the continuous case can be modified for the binary case. The information under the null model would not change. However, the effect size, $\tau$, under the alternative model is not a random variable anymore; it is a fixed value unlike the alternative version of the continuous case. Therefore, $Y_l \sim N(\tau, 1)$ and $P(Y_l > t) = 1 - F_1(t, \tau) = \Phi(\tau - t)$.

## 3. Estimating the distribution of power across tests

### 3.1. Estimating the distribution of power

Consider a multiple hypothesis testing scenario where there are *m* hypothesis tests with normally distributed test statistics $x_1 \ldots x_m$. For each test *i*, define effect size $\varepsilon_i = \sqrt{n}\mu_i/\sigma_i$, where $x_i \sim N\left(\mu_i, \sigma_i/\sqrt{n}\right)$. Assume that tests are ordered so that tests 1 to $m_1$ have $\mu_i$>0. Power for these tests is given by $\bar{\Phi}(Z_\alpha - \varepsilon_i)$, where $Z_\alpha$ is the significance threshold. In the case that the means are zero under the null, then the test statistic $t_i = \bar{x}_i/s_i$ estimates the effect size $\varepsilon_i$. Thus, the power for test *i* can be estimated as $\bar{\Phi}(Z_\alpha - \bar{x}/s)$.

In practice, we estimate $m_1$ from the data using the method of Storey and Tibshirani[1], sort the tests by test statistic or p-value, and then estimate power for the top $m_1$ most significant tests. Because of random variation in test statistic values, the top $m_1$ tests will actually include many null tests. Furthermore, the estimate will be very poor for any single test. However, our goal is to estimate the distribution of power values, not individual values. Take $g(\varepsilon)$ as the distribution of effect sizes. Rather than observing $g(\varepsilon)$, we observe $h(t_i)$, the distribution of effect size estimates. Each effect size estimate $t_i = \bar{x}_i / s_i$ follows a non-central t-distribution with non-centrality parameter $\varepsilon_i = \mu_i / \sigma_i$. The distribution for the effect size estimates can be written as

$$h(t_i) = \int h(t_i \mid \varepsilon_i = \varepsilon) g(\varepsilon) d\varepsilon$$

It is clear that $h(t_i)$ will give a distorted view of $g(\varepsilon)$, depending on the variation of $t_i$ about $\varepsilon_i$. We conducted simulations in in order to explore how well we can estimate the power distribution.

***Simulation procedure.*** We assume that there are a total of $m$=10,000 tests with $m_1$=1000 tests being true effects. The 9,000 null tests have effect size zero, whereas the 1000 alternate hypothesis tests effect sizes follow an exponential distribution. We consider two cases: one where average effect size is 1 and one where it is 4. In the case of one-sided tests, all alternate hypothesis effect sizes have positive signs. In the case of two-sided tests, positive and negative signs were randomly assigned with equal probability.

The true power for each alternate hypothesis tests was calculated as $\bar{\Phi}(z_\alpha - \varepsilon_i)$ for a one-sided test and $\bar{\Phi}(z_\alpha - \varepsilon_i) + \Phi(-z_\alpha - \varepsilon_i)$ for a two-sided test. Test statistic values $t_i$ for each test were generated from a normal distribution with a mean equal to the effect size and standard deviation 1. The tests were sorted by test statistic value for one-sided and absolute value of test statistic for two-sided tests. Then, following our procedure for estimating the power distribution from data, power was estimated for the top $m_1$ tests. Estimated power was calculated as $\bar{\Phi}(z_\alpha - t_i)$ for a one-sided test and $\bar{\Phi}(z_\alpha - t_i) + \Phi(-z_\alpha - t_i)$ for a two-sided test.

If the estimated effect size is opposite from the direction of the one-tailed test, then estimated power is zero. That is, the data shows no evidence of an effect in the hypothesized direction. In these simulations and the estimates of the power distribution from data in the main text, we ignore tests with estimated effect sizes that are negative in order to simplify interpretation of the results.

***Simulation results.*** The resulting true and estimated power distributions for one-sided and two-sided tests are shown in Figures X and Y below. The average effect sizes are 1 and 4, respectively, for Figures X and Y. If sample size were 100 for example, this would correspond to $\mu/\sigma$=0.1 and 0.4, respectively. When the effect size is larger (i.e., the true mean is larger compared to the standard error), then the estimated power distribution matches the true power distribution very well. When the effect size is smaller, then the estimated effect size distribution is biased relative to the true distribution.

For both one-sided and two-sided tests, the estimated power distribution has an excess of higher power tests compared to the true distribution. There are two effects at work: First, when the standard deviation in estimated effect size is large, then estimated effect sizes will frequently have larger magnitude than true effect sizes, and many lower power tests will have estimated power that is higher than their true value. Because there are more low power tests than higher

power ones, the net effect of random variation in estimated effect sizes is that power is overestimated for many tests. The second effect is that there are many more null tests than alternate tests. Many null tests will by chance have higher test statistic values than the true alternate tests – the larger the number of null tests, the larger the number of chance high values. Many of the top $m_1$ tests will be these chance high values. The result of these two effects is that there is a net overestimate of power.

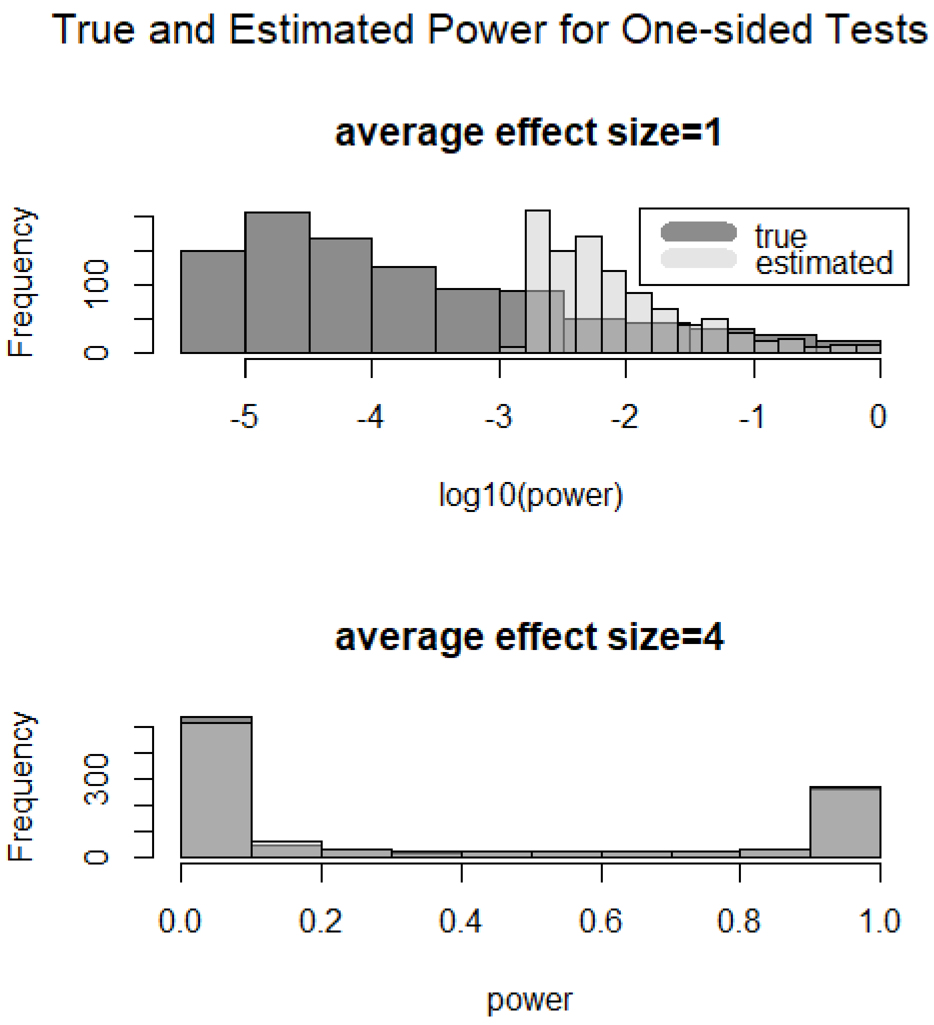


Figure 3.1: True and estimated power distributions for one-sided tests.

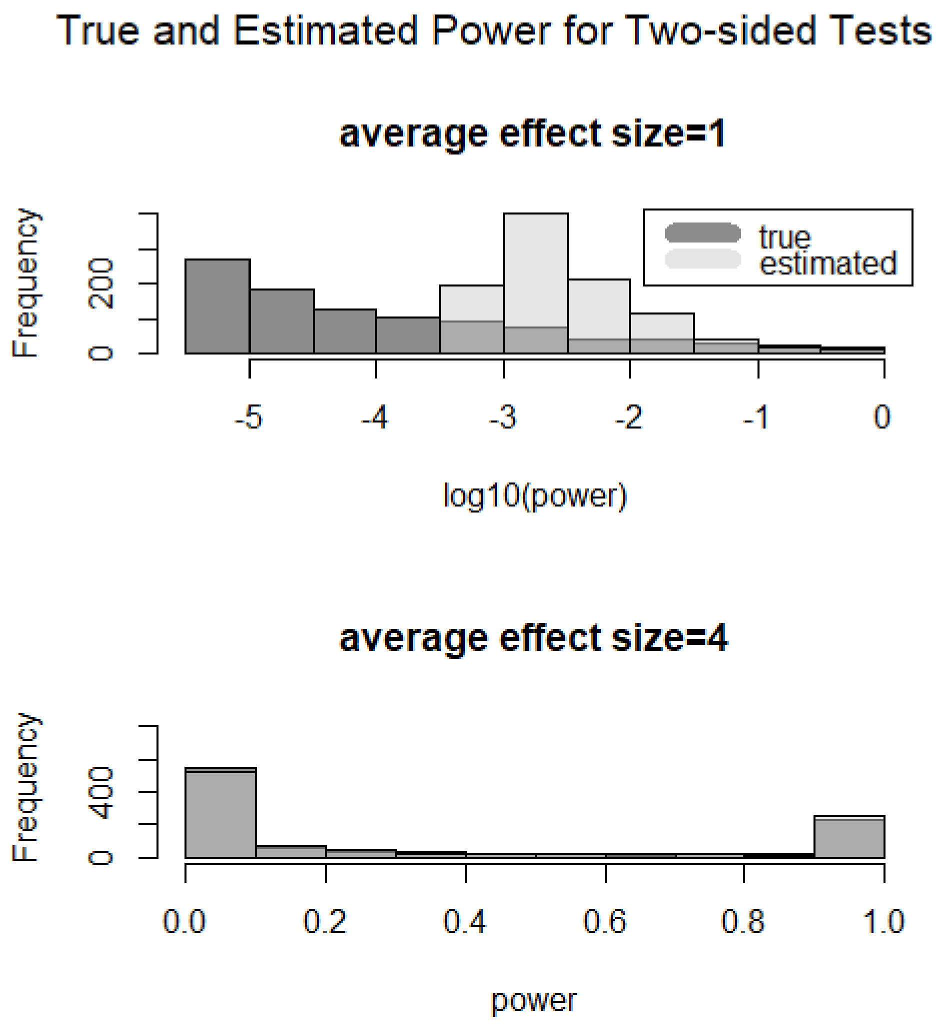


Figure 3.2: True and estimated power distributions for two-sided tests.

**3.2. Efron method for estimating power**

Efron[2] developed a method for power diagnostic for data with many hypothesis tests. As an alternative to the above approach, we will explore this approach as well. In this method, the null distribution $f_0$ of test statistics is estimated from the central part of the empirical distribution near zero. The reasoning is that most test statistics that are near zero should be from the null distribution and thus the distribution of these statistics should approximate the null distribution. Likewise, the alternate hypothesis distribution $f_1$ is estimated from test statistics that are some specified distance away from zero. We used the R package *locfdr* to get the estimated $f_0$ and $f_1$ distributions. From this, we calculated the "thinned counts" following Efron's approach. The test statistics are separated into bins. In each bin $k$, the thinned count is defined as (1-$fdr_k$)*(count for bin $k$), where $fdr_k$ is the estimated local FDR. This gives estimates of the number of alternative hypothesis tests in each bin. We used these counts, along with an estimate of power for each bin, to produce the estimated power distribution for the Bottomly[3] RNA-seq data (Figure 3.3).

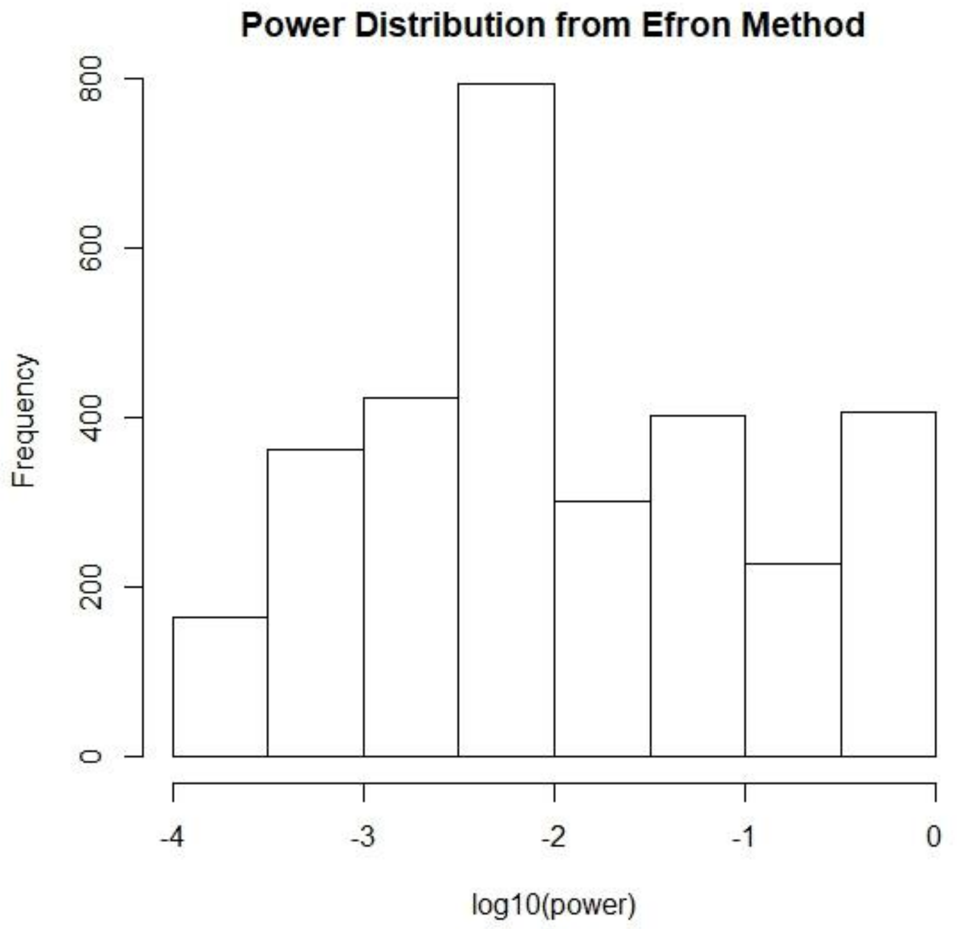


Figure 3.3: Estimated power distribution for Bottomly[3] data using Efron method.

Although the power is still very low for most effects, this distribution is shifted substantially higher than in Figure 1 in the main text. This is largely because the approach of Efron assumes that the central part of the distribution of test statistics is entirely null tests. However, it is likely that effect sizes for many true alternate hypothesis tests are near zero and are thus excluded. This is evident by the fact that the sum of the thinned counts is only 3073, whereas the number of alternate hypothesis tests $m_1$ estimated from the histogram of p-values[1] is 6643.

We explored this via simulations. The simulations were identical to those shown in Figures 3.1 and 3.2 except that power was estimated using Efron's method as described above. Figure 3.4 shows Efron's method is heavily biased towards higher power when there are many low power tests. This is because this method excludes tests with effect sizes near zero. For the scenario shown in the figure, the thinned counts summed to only 482, whereas there were 10,000 hypothesis tests with non-zero effect sizes. Of course, Efron's method focuses on the most important part of the distribution – that is, the tests most likely to be detected – and estimates that effectively. However, it is not effective at capturing the full distribution when there are many tests with very low effect sizes.

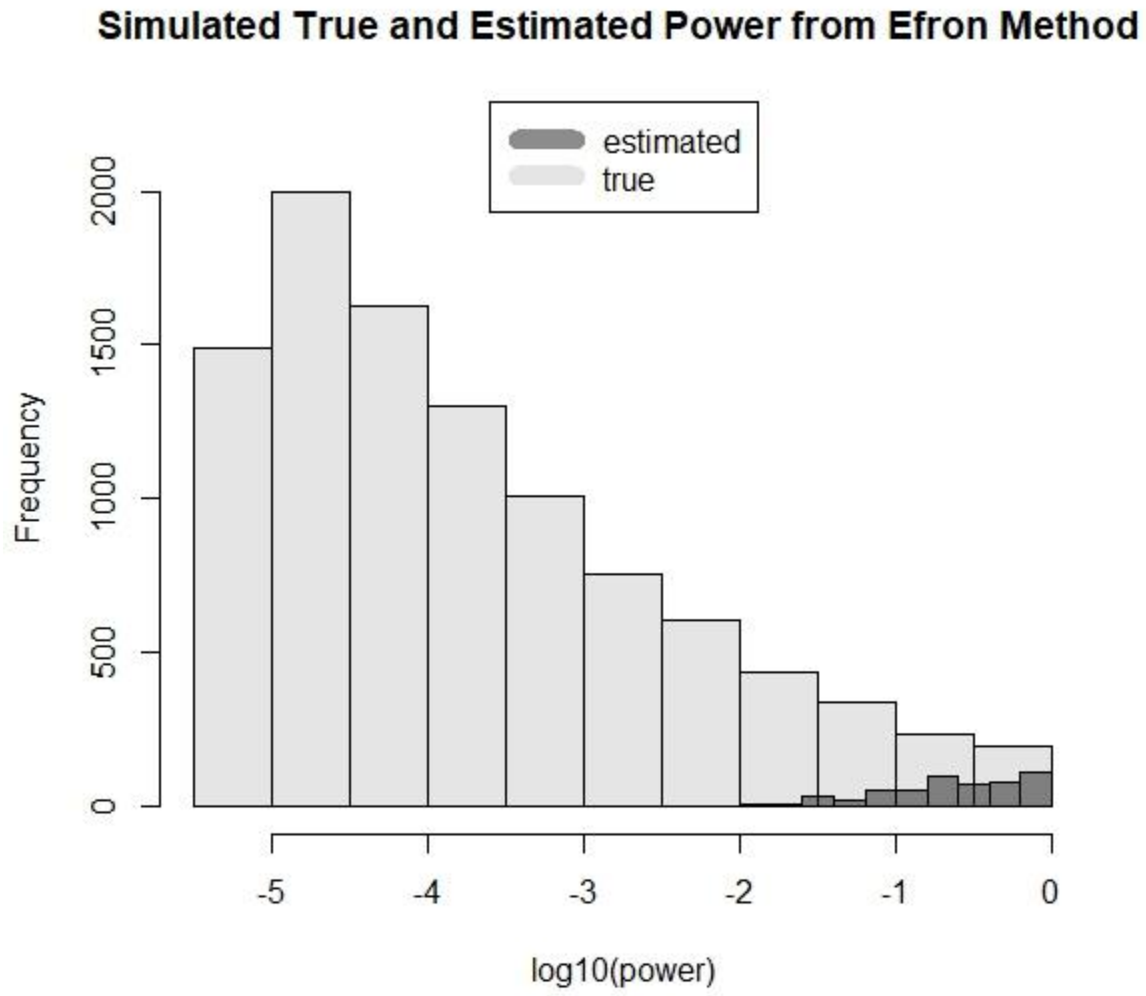


Figure 3.4: Simulation of true and estimated power distribution using Efron's method.

## 4. Simulation Procedures

This section describes how the simulated figures are created in the original article.

### 4.1 Group effect (Figure 2 and Figure 3).

This simulation is conducted to show how alternate tests are washed out by null tests in group-based methods like *IHW*. We chose IHW because *IHW* is the best among the existing group-based methods. To conduct the simulation, we generated $m$ = 40,000 test statistics and covariate statistics from the normal distribution. The mean vector of the statistics is composed of true null and alternative effect sizes, where the proportion of the true nulls $\pi_0$ was prespecified. To see the overall group effect, we ranked the effect sizes by the covariates then split the effect sizes into 10 groups. We then computed the proportion of the true alternative effects ($\varepsilon_i > 0$) in the best group and the mean effect size in the best group. To see the group effect on the IHW method, we applied the *ihw* function from the *R* package *IHW*. For each of the procedures, we conducted 100 replications.

### 4.2 Ranks probability (Figure 4).

A simulation was conducted to verify the proposed method for calculating the ranks probability of tests given effect sizes, $P(r_i = k|\tau_i)$. To perform the simulations, we generated 10,000,000 samples. Each sample is composed of 100 test statistics from the normal distribution with standard deviation 1. We assumed that 50 test statistics are from the null model with effect size 0, and 50 test statistics are from the alternative model. Of these, 49 have effect size $\tau_y \sim uniform(0, 1)$ and one has effect size $\tau_{one} = \{1 \; or \; 2\}$.

We combined both groups of tests by placing the 50 alternative tests first, and the 50 null tests next. We picked the first test (with effect size $\tau_{one}$) and the 51$^{st}$ test and saved their ranks. Since the first test is from the alternative model and 51$^{st}$ test is from the null model, we would expect that the rank of the first test is always higher; however, this may not be always true, especially if the effect size is very low. We followed the same procedure for 10,000,000 samples and computed the relative frequency of the ranks. This gives estimates of the probability for the test to be at each rank by simulation approach. Additionally, Theorem 2 and Proposition 1 compute ranks probability using importance sampling as described in that section for the exact and approximation approach.

### 4.3. Ranks probability and weight (Figure 5).

To calculate the rank probabilities in Figure 5, we applied the proposed normal approximation method (Proposition 1). We assumed that there are $m = 10{,}000$ hypotheses tests; the test statistics follow normal distributions with mean 0 and $\varepsilon_i$ under the null and alternative models, respectively, and standard deviations 1.

To calculate the corresponding normalized weight, we applied the rank probabilities in the weight formula (Theorem 1) and then numerically optimized with respect to the Lagrangian multiplier $\delta$ so that weights sum to $m$. For additional plots see SI section 8.

### 4.4. Power (Figures 6 and 7).

We used simulations to compare the statistical performance of four methods: the Benjamini and Hochberg[4] FDR procedure with no weighting (BH), the weighting method of

Roeder and Wasserman[5], the Independent Hypothesis Weighting[6] (IHW), and our proposed CRW method.

Simulated data were generated for various scenarios and used to estimate power, FDR, and FWER for each method. The simulations for power were divided into three groups based on the proportion of the true null hypothesis. The three groups were composed of $50\%, 90\%$, and $99\%$ true null tests. For each group of simulations, we considered the combination of correlations × effect sizes = $\{0,\ .3,\ .5,\ .7,\ .9\} \times \{E(\varepsilon_i) = E(\tau_i),\ E(\varepsilon_i) \sim N(E(\tau_i),\ CV.E(\tau_i))\}$, where $E(\varepsilon_i), E(\tau_i)$, and $CV$ refers to the mean test-effect, mean covariate-effect, and coefficient of variation. The correlation was between test statistics. For the mean effect sizes and the CV, we considered a vector of $\{.2,\ .4,\ .6,\ .8,\ 1,\ 2,\ 3,\ 8\}$ and $CV = \left\{0,\ \frac{1}{2},\ 1,\ 3,\ 10\right\}$. Different $CV$ were used to take into account the influence of the variance of the effect sizes. When the $CV = 0$, we kept the mean test and the mean covariate effect the same; however, for the other cases the mean test-effects were generated from the normal distribution with mean $E(\tau_i)$ and standard deviation $CV.E(\tau_i)$.

For the non-correlated and correlated cases, we generated tests from the normal distribution and the multivariate normal distribution, respectively. The correlation matrix of the multivariate normal distribution had 10,000 rows and 10,000 columns; however, the matrix is diagonally split into 100 blocks, and each block consists of 100 rows and 100 columns. All the remaining cells are filled with zeros. Thus, the hypothesis tests were assumed to be structured as 100 blocks each with 100 correlated tests. This type of structure might be observed, for example, with correlated expression in gene expression data or linkage disequilibrium between correlated markers in a genome-wide association study (GWAS). We conducted simulation of 1,000 replicates and assumed that there were $m = 10{,}000$ hypotheses tests. For each replicate, we determined the proportion of true positive results then calculated the average across the replicates. To see the power for the binary effect size, see SI section 11. For other simulations, such as FWER and FDR, we adapted the similar procedures (see section 9 and section 10 in SI).

To obtain the results corresponding to the BH method, we used $p.adjust$ function from $R$ software and followed the Benjamini and Hochberg FDR procedure[4]. To implement the RDW method and estimate the weights, we followed the procedures described in the paper[5], section 5; and to implement the $IHW$ method, we applied the $ihw$ function from the R (or Bioconductor) package $IHW$ and kept the default settings.

**5. Work Flow**

The steps of our workflow are given below:

**Data Analysis.** Before applying CRW, we performed a pre-screening analysis of the data composed of p-values $(P)$ and the covariates $(Y)$. We then followed several steps to analyze the data, in particular, to obtain the ranks probability, $P(r_i = k | E(\varepsilon_i))$ and the corresponding weights $w_i$. The steps are summarized below:

**Input:** A nominal significance level $\alpha \in (0, 1)$, a vector of p-values $P = p_1, \dots \dots \dots, p_m$ and a vector of covariates $Y = y_1, \dots \dots \dots, y_m$ corresponding to each p-value, which is independent of $P$ under $H_0$.

Step 1: Denote the vector of test statistics by $T$. Obtain the test statistics by $T = \Phi^{-1}(1-P)$ for the one-tailed and $T = \Phi^{-1}\left(1-\frac{P}{2}\right)$ for the two-tailed p-values, where $\Phi^{-1}(.)$ refers to the inverse of the standard normal Cumulative Density Function (CDF).

Step 2: Define a simple linear regression by $y_i = \beta_0 + \beta_1 t_i + \epsilon; 1 = 1, \dots \dots \dots, m$. Obtain the relationship between the test statistics $(T)$ and the covariates $(Y)$ by the linear regression. In the regression, Box-Cox transformation or other transformations need to be used if the covariates are not approximately normal.

Step 3: Denote by $m, m_0$, and $m_1$ the number of hypothesis tests, the number of true null tests, and the number of true alternative tests, respectively. Estimate the numbers of the tests by using the method of Storey and Tibshirani[1]. In particular, use the *qvalue* function from the R package *qvalue*.

Step 4: Order the test statistics in the decreasing order and pick the top $m_1$ tests. This set of tests is used to estimate the alternative hypothesis test effects.

Step 5: Denote by $\bar{T}$ and $T_m$ the mean and the median of the true alternative test statistics. Calculate these from the top $m_1$ tests from Step 4.

Step 6: Apply the estimated model $\hat{y}_i = \hat{\beta}_0 + \hat{\beta}_1 t_i$ to compute the predicted covariates $\hat{Y}$ and $\hat{Y}_m$ for the mean and the median test statistics. The predicted covariates corresponding to the mean and the median tests statistics were considered as the estimate of the mean covariate-effect sizes.

Step 7: Apply Theorem 2 to compute the ranks probability $P(r_i = k|E(\varepsilon_i))$, where $E(\varepsilon_i)$ will be replaced by the value of $\hat{Y}$ and $\hat{Y}_m$ if the effects are assumed continuous and binary, respectively.

Step 8: Compute weights by applying Theorem 1 or Corollary 2, where $E(\varepsilon_i)$ will be replaced by $\bar{T}$ and $T_m$ if the effects are assumed continuous and binary, respectively.

Step 9: Apply the weighted Bonferroni method $\sum_{i=1}^{m} I\left(p_i \leq \frac{\alpha w_i}{m}\right)$ or weighted FDR in the Benjamini and Hochberg[7] procedure $\sum_{i=1}^{m} I(p_{ia} \leq \alpha)$ to obtain the number of significant tests, where $I(.)$ and $p_{ia}$ refers to the indicator function and the adjusted p-values after applying the weights, i.e., $p_{ia} = adjust\left(\frac{p_i}{w_i}\right)$, respectively.

Note that, the diagnostic plots of the data suggested that the regression models did not fit well. A pin-point model diagnosis process can improve the fitness of the models. This leaves a scope of further research, which is beyond the goal of this article. However, the current model information is sufficient for our present purposes, because CRW only requires the centers of the test-effect sizes and the corresponding covariate-effect sizes.

**Code availability.** Two R packages are available on GitHub to reproduce the results: 1) *OPWeight* and 2) *OPWpaper*. The packages come with detailed documentation and vignettes that show the application procedures of CRWs. The executable documents, code, and results of

the data and the simulations can be obtained from https://github.com/mshasan/OPWeight or Bioconductor link: https://bioconductor.org/packages/release/bioc/html/OPWeight.html and https://github.com/mshasan/OPWpaper.

## 6. Additional proofs

**a. Compute $\boldsymbol{P(Y_l > t)}$.** Suppose the test statistic, $Y_l$, under the alternative model is from a normal distribution, i.e., $Y_l \sim N(\tau_l, 1)$, where $\tau_l$ is a random variable of the effect size; then $P(Y_l > t) = 1 - \int F_1(t, \tau_l) f(\tau_l) d\tau_l = 1 - \int \Phi(t - \tau_l) f(\tau_l) d\tau_l$, where $f(\tau_l)$ is the probability density function of $\tau_l$.

**i)** If the effect size is $\tau_l \sim uniform\ (a, b)$, then $P(Y_l > t)$ is computed as:

$$P(Y_l > t) = \frac{1}{b-a} \int_a^b \Phi(\tau_l - t) d\tau_l.$$

Let $x = \tau_l - t$; then by applying integration by parts we have

$$P(Y_l > t) = \frac{1}{b-a} \int_{a-t}^{b-t} \Phi(x) dx = \frac{1}{b-a} [x\Phi(x) + \phi(x)]_{a-t}^{b-t}$$

$$= \frac{1}{b-a} [(b-t)\Phi(b-t) - (a-t)\Phi(a-t) + \phi(b-t) - \phi(a-t)].$$

**ii)** If the effect size is $\tau_l \sim Normal\ (\eta,\ \sigma^2)$, then $P(Y_l > t)$ is computed as:

$$P(Y_l < t) = \int \Phi(t - \tau_l) \frac{1}{\sigma}\ \phi\left(\frac{\tau_l - \eta}{\sigma}\right) d\tau_l.$$

Denote $\frac{dP(Y_l < t)}{dt} = \frac{dp}{dt}$. Differentiating w.r.t $t$ produces

$$\frac{dp}{dt} = \int \phi(t - \tau_l) \frac{1}{\sigma}\ \phi\left(\frac{\tau_l - \eta}{\sigma}\right) d\tau_l.$$

For simplicity, denote $x = \frac{\tau - \eta}{\sigma}$, thus $dx = \frac{d\tau_l}{\sigma}$. Then, after rearranging the parameters and performing algebraic manipulations, we obtain

$$\frac{dp}{dt} = \int \frac{1}{\sqrt{\left(\frac{1}{\sigma^2+1}\right)}} \phi\left(\frac{x - \frac{\sigma t - \sigma\eta}{\sigma^2+1}}{\sqrt{\left(\frac{1}{\sigma^2+1}\right)}}\right) dx. \frac{1}{\sqrt{\sigma^2+1}}\ \phi\left(\frac{t-\eta}{\sigma^2+1}\right).$$

The first part is the normal pdf. Therefore integration to this is 1, which reduces to

$$\frac{dp}{dt} = \frac{1}{\sqrt{\sigma^2+1}}\ \phi\left(\frac{t-\eta}{\sigma^2+1}\right).$$

Integrating $\frac{dp}{dt}$ w.r.t $t$ produces a normal CDF. Therefore,

$$P(Y_l > t) = 1 - \Phi\left(\frac{t-\eta}{\sigma^2+1}\right).$$

**iii)** If the effect the size $\tau_l \sim exponential\ (\lambda)$, then $P(Y_l > t)$ is computed as:

$$P(Y_l > t) = \int_0^\infty \Phi(\tau_l - t) \lambda e^{-\lambda \tau_l} d\varepsilon_l$$

Let $x = \tau_l - t$; then we have

$$= \int_{-t}^{\infty} \Phi(x)\lambda e^{-\lambda(x+t)} dx = e^{-\lambda t} \int_{-t}^{\infty} \Phi(x)\lambda e^{-\lambda x} dx.$$

Applying the integration by parts provides

$$= e^{-\lambda t} \left[ \Phi(x) \int \lambda e^{-\lambda x} dx - \int \left( \frac{\mathrm{d}}{dx} \Phi(x) \int \lambda e^{-\lambda x} dx \right) dx \right]_{-t}^{\infty}.$$

After simple integration and algebraic manipulation, we obtain

$$P(Y_l > t) = \Phi(-t) + e^{-\lambda t} e^{\frac{\lambda^2}{2}} \Phi(t - \lambda).$$

**b. Relationship between covariate and test effects.**

Suppose $X$ = test effect, and $Y$ =covariate effect; then

$$E(P(r|Y)|X) = E\left( \frac{P(r,Y)}{f(Y)} |X \right) = E\left( \frac{P(Y|r)P(r)}{f(Y)} |X \right).$$

$Y$ is a random variable depending on $X$, but $r$ is fixed; therefore, this expectation is conducted with respect to the pdf of $Y$ given $x$. Thus,

$$E\left( \frac{P(Y|r)P(r)}{f(y)} |X \right) = \int \left( \frac{P(y|r)P(r)}{f(y)} |X \right) f(y|x) dy = \int P(r|y) f(y|x) dy.$$

Because $X$ is already conditioned in the pdf, $f(y|x)$, there is no need to include x again. Therefore,

$$E(P(r|Y)|X) = \int P(r|y) f(y|x) dy = P(r|X).$$

**c. Weight for the two-tailed p-values.**

The likelihood equation for the two-tailed test can be expressed as

$$L(w_i; r_i) = \frac{2}{m} \sum_{i=1}^{m} \int \bar{\Phi} \left( Z_{\frac{\alpha w_i}{2m}} - \varepsilon \right) m P(r_i|\varepsilon) f(\varepsilon_i)\, d\varepsilon - \delta \left( \frac{1}{m} \sum_{i=1}^{m} w_i - 1 \right).$$

Differentiating the likelihood equation with respect to $w_i$ produces

$$\frac{dL}{dw_i} = \frac{2}{m} \int_{\varepsilon_i=0}^{\infty} \frac{-\phi\left( \bar{\Phi}^{-1}\left( \frac{\alpha w_i}{2m} \right) - \varepsilon \right) \left( \frac{\alpha}{2m} \right)}{-\phi\left( \bar{\Phi}^{-1}\left( \frac{\alpha w_i}{2m} \right) \right)} m P(r_i|\varepsilon) f(\varepsilon) d\varepsilon - \frac{\delta}{m}.$$

After equating $\frac{dl}{dw_k}$ = 0 and performing simple algebra, we obtain

$$\int \left( e^{Z_{\frac{\alpha w_k}{2m}} \varepsilon - \frac{\varepsilon^2}{2}} \right) P(r_i|\varepsilon) f(\varepsilon) d\varepsilon = \frac{\delta}{\alpha}.$$

Suppose

$$g(\varepsilon) = \left(e^{\frac{Z_\alpha w_i}{2m}\varepsilon - \frac{\varepsilon^2}{2}}\right) P(r_i|\varepsilon_i).$$

Since $\varepsilon$ is a random variable, and $g(\varepsilon)$ is differentiable, by the first order Taylor series expansion of $g(\varepsilon)$, we have $E(g(\varepsilon)) \approx g(E(\varepsilon))$. Consequently, the above equation reduces to

$$E\big(g(\varepsilon)\big) \approx \left(e^{\frac{Z_\alpha w_i}{2m}E(\varepsilon) - \frac{E(\varepsilon)^2}{2}}\right) P(r_i|E(\varepsilon)) \approx \frac{\delta}{\alpha}.$$

Consequently, an approximate version of the weight can be obtained, which is

$$w_i \approx \left(\frac{2m}{\alpha}\right) \bar{\Phi}\left(\frac{E(\varepsilon)}{2} + \frac{1}{E(\varepsilon)} log\left(\frac{\delta}{\alpha P(r_i|E(\varepsilon))}\right)\right).$$

**7. Ranks probability of test given effect size, $P(r_i = k|\tau_i)$.**

The probability of rank of the test given the effect size refers to the probability of a particular test being higher than any other test when the effect size is known. In this section, we show the properties of the probability of the rank from three different approaches: 1) Simulation approach 2) Exact numerical solution of the CRW method, and 3) Normal approximation of the CRW method, for both the binary and the continuous effect sizes. We included the simulation approach to verify the CRW methods of $P(r_i = k|\tau_i)$.

We proposed that the probability of the rank can be obtained by using the following exact formula:

$$P(r_i = k|\tau_i) = \sum_{k_0=1}^{k} E_T\{P(r_{1i} = k - k_0 + 1|\tau_i, t) P(r_{i0} = k_0|\tau_i, t)\},$$

where

$$P(r_{1i} = k - k_0 + 1|\tau_i, t) = \begin{cases} \binom{m_1}{k - k_0} (1 - F_1)^{k-k_0} F_1^{m_1-(k-k_0)} \; if\; \tau_i = 0 \\ \binom{m_1 - 1}{k - k_0} (1 - F_1)^{k-k_0} F_1^{(m_1-1)-(k-k_0)} if\; \tau_i > 0 \end{cases},$$

and

$$P(r_{i0} = k_0|\tau_i, t) = \begin{cases} \binom{m_0 - 1}{k_0 - 1} (1 - F_0)^{k_0-1} F_0^{m_0-k_0} \; if\; \varepsilon_i = 0 \\ \binom{m_0}{k_0 - 1} (1 - F_0)^{k_0-1} F_0^{m_0-(k_0-1)} \; if\; \tau_i > 0 \end{cases},$$

where $\tau_i = 0$ under the null hypothesis and $\tau_i = \tau$ for the binary effect and $\tau_i > 0$ for the continuous effect under the alternative hypothesis. This equation, $P(r_i = k|\tau_i)$, is not easily tractable and finding a closed form solution is difficult. However, this equation can be solved numerically and can also be easily simulated. We solved this equation using the importance sampling method of the Monte Carlo (MC) simulation; however, this approach is not fast enough to handle a large number of tests. We propose a normal approximation as an alternative approach to solving the equation, which is expressed as

$$P(r_i = k|\tau) = \begin{cases} E_T N(\mu_0, \sigma_0^2), \; if \tau_i = 0 \\ E_T N(\mu_1, \sigma_2^2), \; if \tau_i > 0 \end{cases},$$

where

$$\mu_0 = (m_0 - 1)(1 - F_0) + m_1(1 - F_1) + 1$$
$$\mu_1 = m_0(1 - F_0) + (m_1 - 1)(1 - F_1) + 1$$
$$\sigma_0 = (m_0 - 1)(1 - F_0)F_0 + m_1(1 - F_1)F_1$$
$$\sigma_1 = m_0(1 - F_0)F_0 + (m_1 - 1)(1 - F_1)F_1.$$

where $F_0$ is the cumulative density function of the statistic $X_j$ under the null model, i.e, $\tau_i = 0$; and $F_1$ is the cumulative density function of the statistic $Y_l$ under the alternative model, i.e, $\tau_i > 0$. In this article, we assumed that $F_0$ and $F_1$ are from the normal distributions.

**7.1. $P(r_i = k|\tau_i)$ given continuous effect.**

Suppose there are $m$ hypotheses tests of which $m_0$ tests are from the true null models, and $m_1$ tests are from the true alternative models, and the test statistics are normally distributed with mean $\tau_i$ and standard deviation 1. We want to test $H_0: \tau_i = 0$ vs. $H_1: \tau_i > 0$; $i = 1, \dots \dots 100$, where $\tau_i$ is a continuous random variable. Our goal is to compute the probabilities of the ranks of the test statistics from three approaches mentioned earlier.

**a. Simulation approach.** To perform the simulations, we generated 10,000,000 samples; each sample is composed of 100 test statistics from the normal distribution for a particular combination of the effect sizes $\{0\} \times Uniform(a,\ b)$, where $\{0\}$ represents the effect size of the null model, and $Uniform(a,\ b)$ represents the effect sizes of the alternative models. We consider the combination of $a = \{0,1\}$ and $b = \{1, 2\}$, respectively. For each sample, we assumed that there are $m = 100$ hypotheses tests of which $m_0 = \{20, 50, 75, 90, 99\}$ tests are from the null, and $m_1 = \{80,\ 50, 25, 10, 1\}$ tests are from the alternative models, respectively. For example, if we are interested in testing the hypothesis $H_0: \tau_i = 0$ vs. $H_1: \tau_i > 0$; $\tau_i \sim uniform(0, 1)$; $i = 1, \dots \dots, 100$, and we assumed that 50 tests are from the null, and 50 tests are from the alternative models, then the simulation parameters will be $a = 0,\ b = 1,\ m = 100,\ m_0 = 50$ and $m_1 = 50$. That is, 50 test statistics are from the normal distribution (null model) with mean 0 (effect size 0) and standard deviation 1, and the remaining 50 test statistics are from the normal distribution (alternative model) with mean $uniorm(0, 1)$ and standard deviation 1. Then, we combined both groups of tests by placing the 50 alternative tests first, and the 50 null tests later. We picked the first test and the 51st test and saved their ranks. Since the first test is the true alternative and 51st test is the true null, we would expect that the rank of the first test is always higher; however, this may not be always true, especially if the effect size is very low. We followed the same procedure for 10,000,000 samples and computed the relative frequency of the ranks, which are the ultimate the probabilities of the ranks of the tests by the simulation approach. For simplicity, we considered test statistics to be normally distributed with mean $\tau_i = 0$ and $\tau_i > 0$ under the null and alternative models, respectively, and standard deviation 1. That is, $F_0$ and $F_1$ are the cumulative functions of the normal distributions. One can easily expand the idea to other distributions.

**b. Exact and Normal approximation approach.** For the CRW methods (both the exact and the normal approximation), we performed Monte Carlo (MC) simulations by considering the importance sampling approach. We considered 100,000 replications in the MC simulation to obtain smother probability curves; however, most of the time 10,000 replications will provide the similar results. For the CRW method, we followed similar procedures regarding the parameters described in the simulation approach. In addition, we directly computed $F_0$ and $F_1$ from $F_0 =$

$P(X_j > t) = \Phi(-t)$ and $F_1 = P(Y_l > t) = \frac{1}{b-a}[(b-t)\Phi(b-t) - (a-t)\Phi(a-t) + \phi(b-t) - \phi(a-t)]$, respectively, to obtain the binomial probability of a test being higher than a specific test $t$.

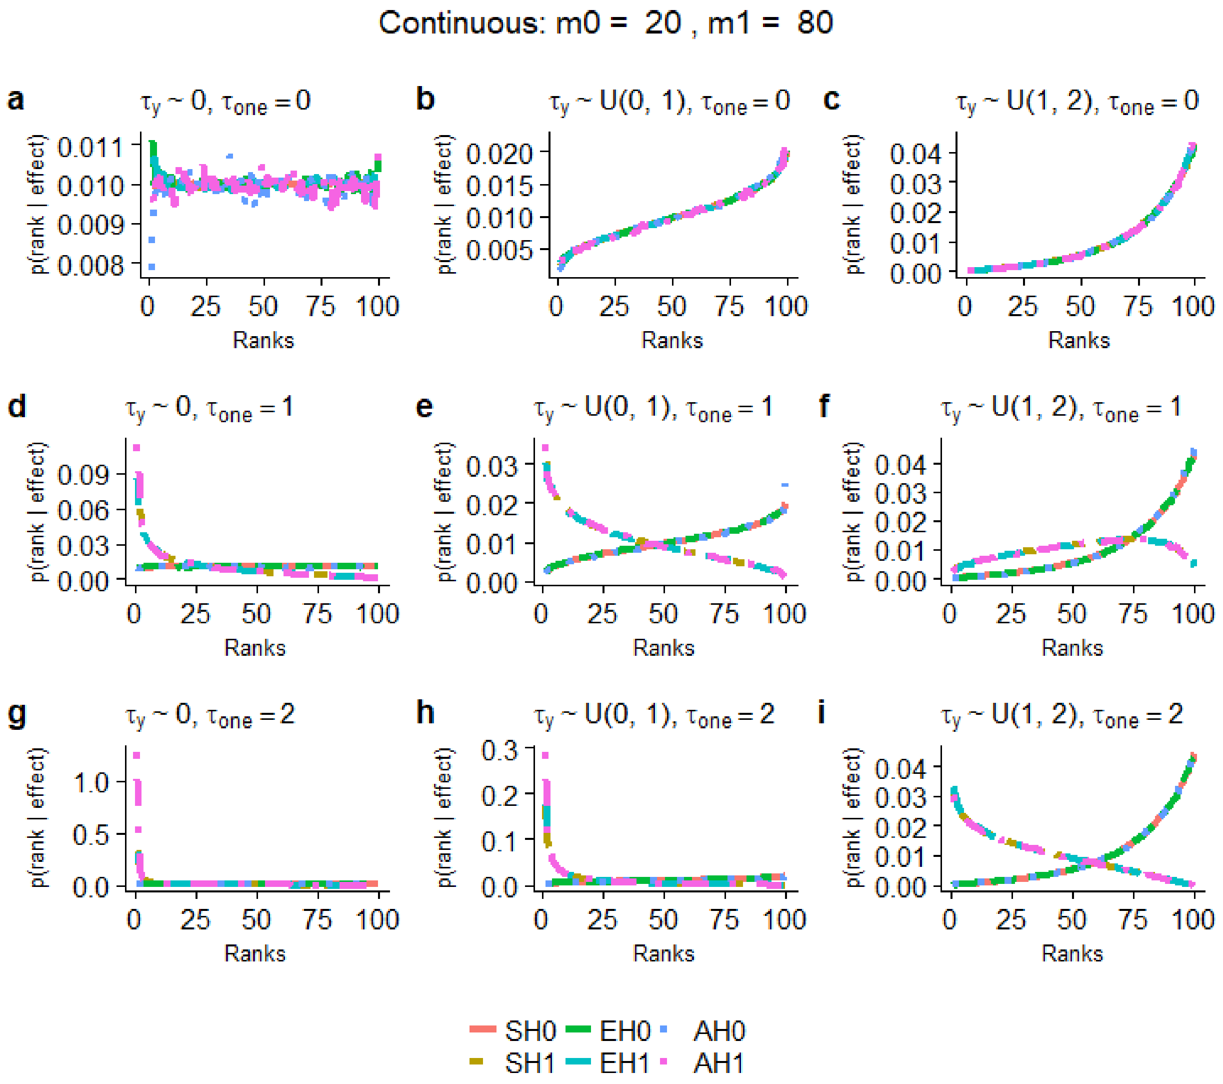


**Figure 7.1.1:** This Figure shows $P(r_i = k|\tau_i)$ for the continuous case for three different scenarios: 1) from the simulation, 2) from the exact CRW method, and 3) from the CRW normal approximation. To generate these plots, we assumed that there are $m = 100$ tests of which $m_0 = 20$ are true nulls, and $m_1 = 80$ are true alternatives. The true null tests have mean 0 and the true alternate tests have the distribution $\tau_y$ as shown at the top of each plot Each plot consists of six curves, SH0, SH1, EH0, EH1, AH0, and AH1, where the first letter represents the method (S = simulated, E = exact, and A = approximate), and H0 and H1 represent the hypothesis type. Three curves (SH0, EH0, and AH0) starting from the bottom-left represent $P(r_i = k|\tau_i = 0)$, and the remaining three curves (SH1, EH1, and AH1) starting from top-left represent $P(r_i = k|\tau_i = \tau_{one})$, where $\tau_{one} = \{0,1,2\}$. All the curves show the probability of the rank of a statistic with effect size either $\tau_i = 0$ or $\tau_i = \tau_{one}$ across all tests. For example, for the curves of the sixth plot (starting from left-right), there are 20 test statistics from the null models

with effect size 0; 79 test statistics with effect size $\tau_y \sim uniform(1,2)$ and one test statistic with the effect size $\tau_{one} = 1$ are from the alternative models. Thus, the curves SH1, EH1, and AH1 show the probability of the alternative test statistic with effect size $\tau_{one} = 1$ being higher in rank than the other test statistics, and SH0, EH0, and AH0 show the probability of a null test statistic with effect size $\tau_i = 0$ being higher in rank than the other test statistics. All plots of the simulation suggest nearly perfect alignment with the CRW (exact and approximate) methods.

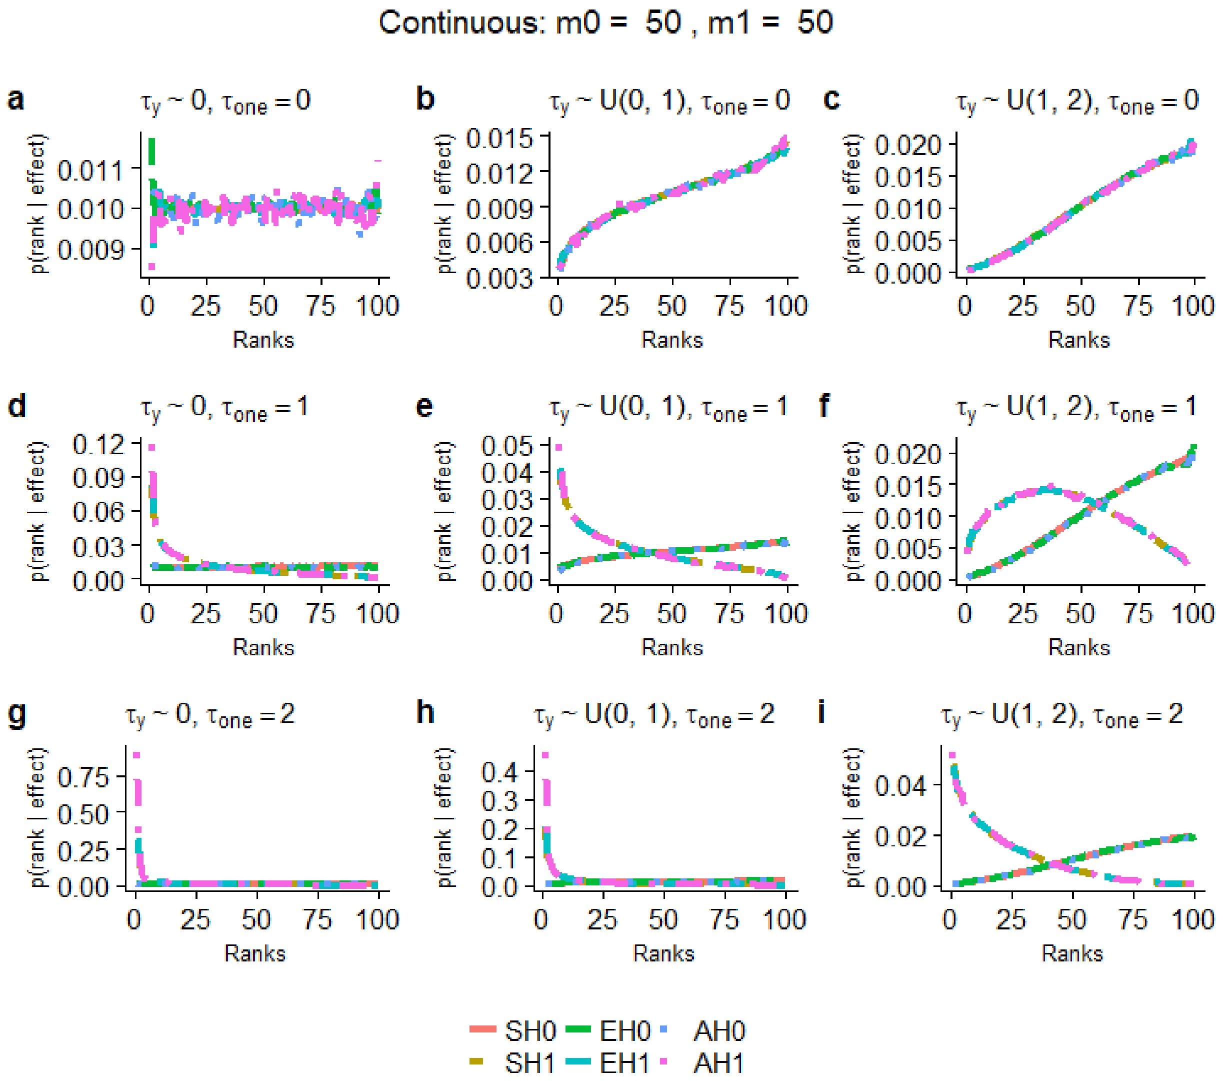


**Figure 7.1.2:** This Figure shows $P(r_i = k|\tau_i)$ for the continuous case in three different scenarios. To generate these plots, we assumed that there are $m = 100$ tests of which $m_0 = 50$ are true nulls and $m_1 = 50$ are true alternatives.

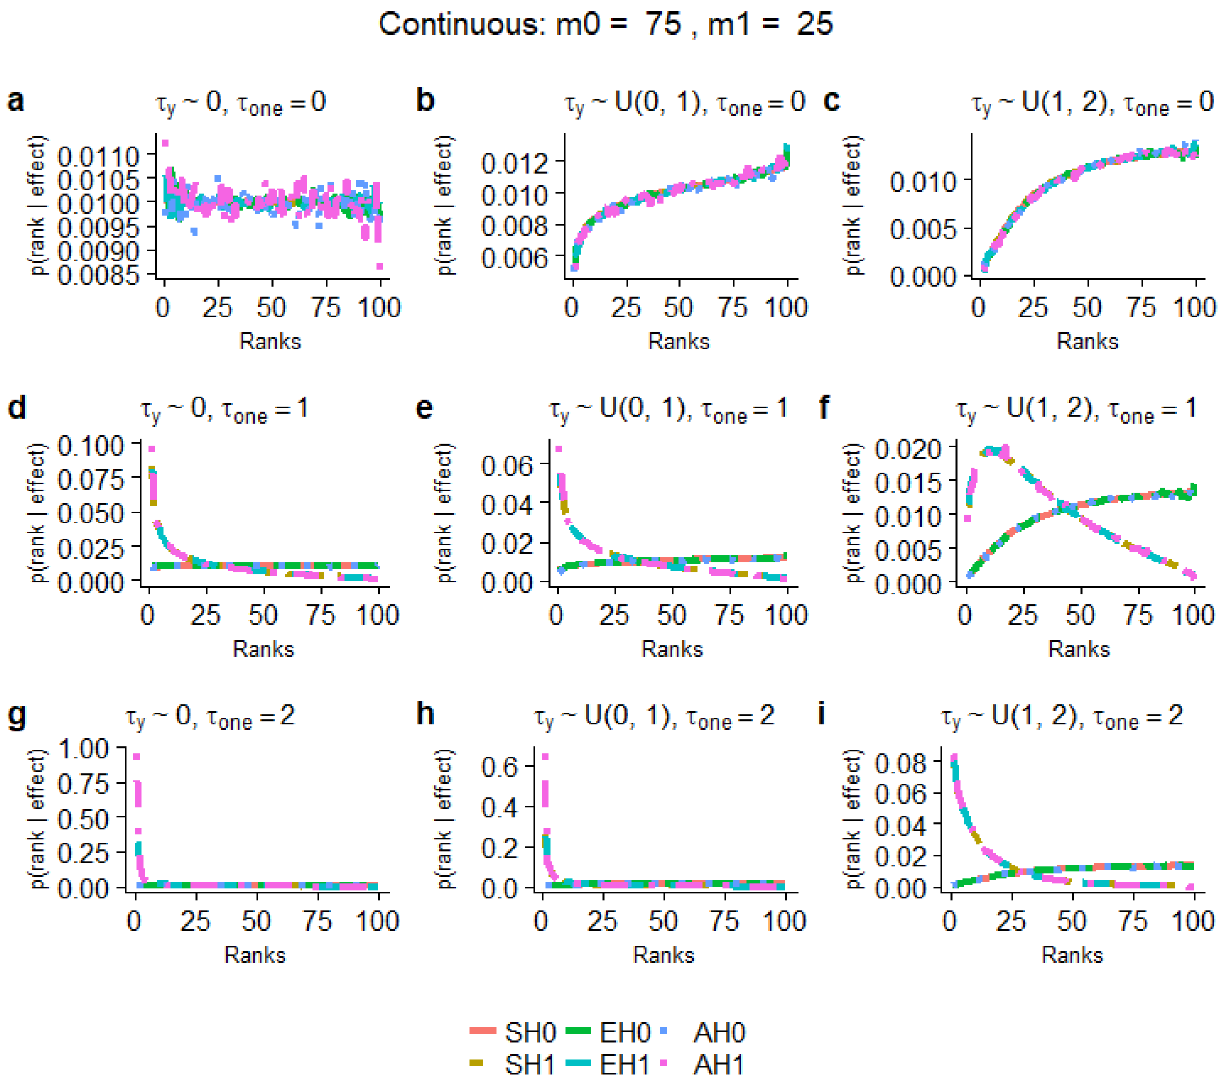


**Figure 7.1.3:** This Figure shows $P(r_i = k|\tau_i)$ for the continuous case in three different scenarios. To generate these plots, we assumed that there are $m = 100$ tests of which $m_0 = 75$ are true nulls and $m_1 = 25$ are true alternatives.

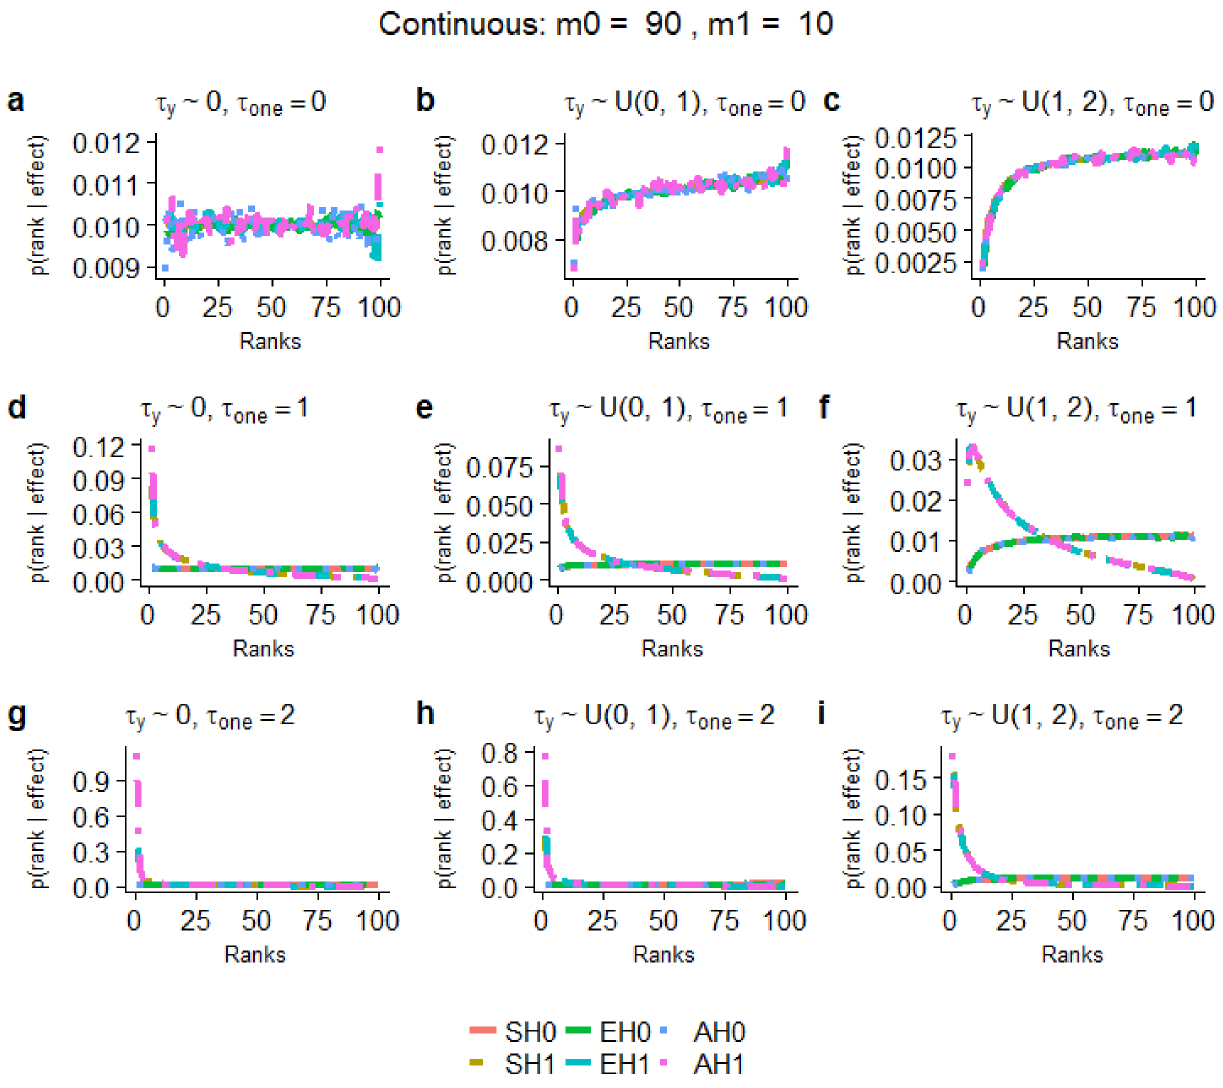


**Figure 7.1.4:** This Figure shows $P(r_i = k|\tau_i)$ for the continuous case in three different scenarios. To generate these plots, we assumed that there are $m = 100$ tests of which $m_0 = 90$ are true nulls and $m_1 = 10$ are true alternatives.

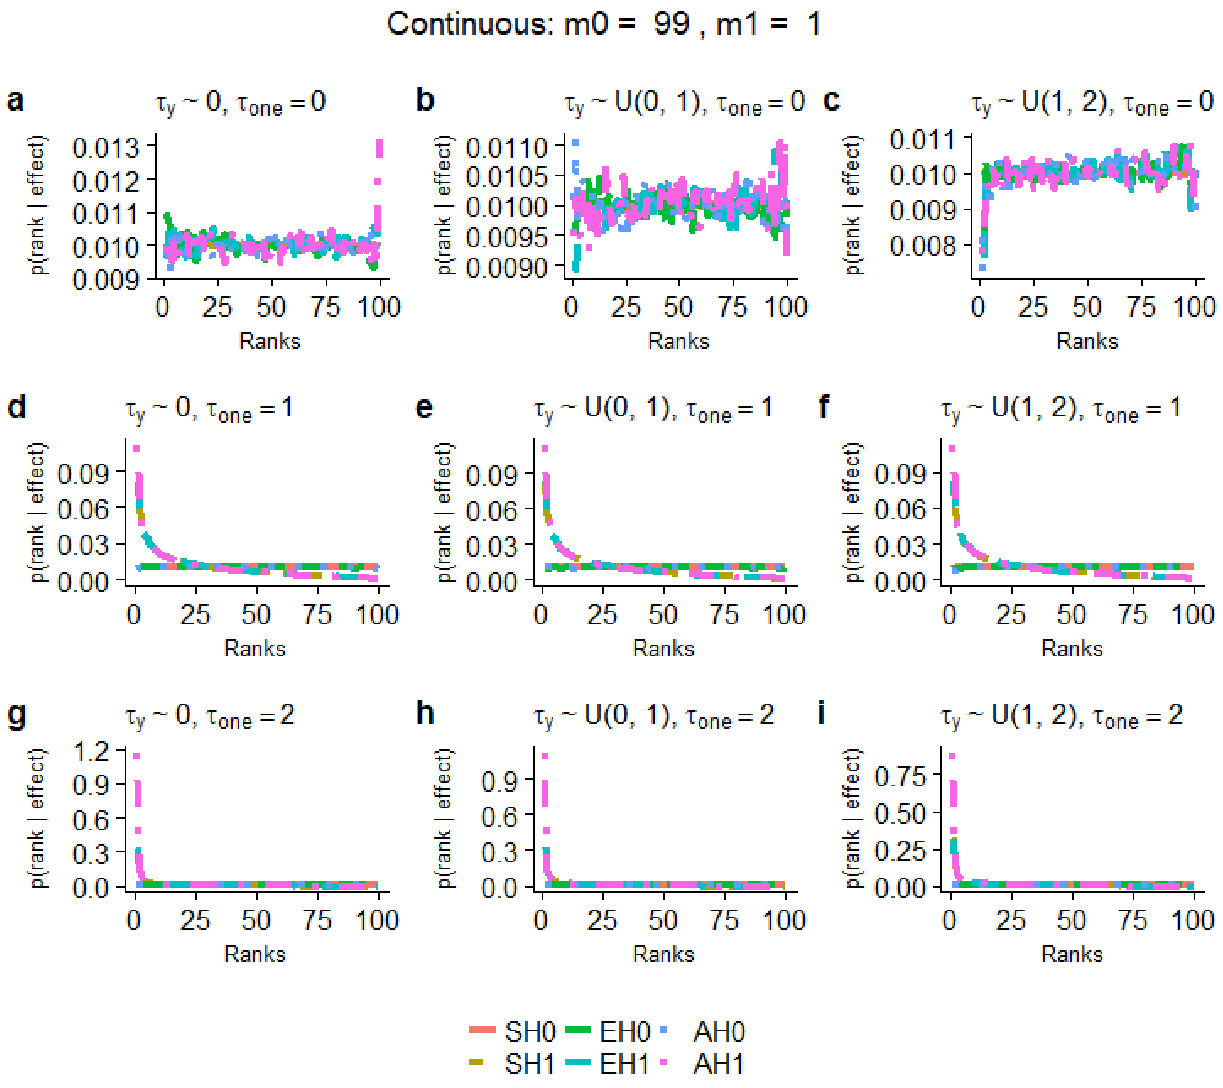


**Figure 7.1.5:** This Figure shows $P(r_i = k|\tau)$ for the continuous case in three different scenarios. To generate these plots, we assumed that there are $m = 100$ tests of which $m_0 = 99$ are true nulls and $m_1 = 1$ are true alternatives.

### 7.2. $P(r_i = k|\tau_i)$ given binary effect.

Suppose there are $m$ hypotheses tests of which $m_0$ tests are from the true null models, and $m_1$ tests are from the true alternative model, and the test statistics are normally distributed with mean $\tau_i$ and standard deviation 1. We want to test $H_0: \tau_i = 0$ vs. $H_1: \tau_i = \tau;\ i = 1, \ldots \ldots 100$, where $\tau$ is a fixed value. Our goal is to compute the probabilities of the ranks of the test statistics from three approaches mentioned earlier.

**a. Simulations approach.** To perform the simulations, we generated 10,000,000 samples; for a particular combination of the effect sizes $\{0\} \times \{0,1,2\}$, where $\{0\}$ represent the effect size of the null, model and $\{0,1,2\}$ represents the effect sizes of the alternative models. For each sample, we assumed that there are $m = 100$ hypotheses tests of which $m_0 =$

$\{20, 50, 75, 90, 99\}$ tests are from the null, and $m_1 = \{80,\ 50, 25, 10, 1\}$ tests, respectively, are from the alternative models. For example, if we are interested in testing the hypothesis $H_0: \tau_i = 0$ vs. $H_1: \tau_i = 1$, and we assumed that 50 tests are from the null, and 50 tests are from the alternative models, then the simulation parameters will be $m = 100$, $m_0 = 50$ and $m_1 = 50$. That is, 50 tests are from the normal distribution with effect size 0 (null model) and 50 tests are from the normal distribution with common effect size 1 (alternative model). For simplicity, we considered test statistics to be normally distributed with mean $\tau_i = 0$ and $\tau_i = \tau$ under the null and alternative models, respectively, and standard deviation 1. That is, $F_0$ and $F_1$ are the cumulative functions of the normal distributions.

We combined both groups of tests by placing the 50 alternative tests first, and the 50 null tests later. We picked the first test and the $51^{st}$ test and saved their ranks. Since the first test is the true alternative and the $51^{st}$ test is the true null, we would expect that the rank of the first test is always higher; however, this may not always be true, especially if the effect size is very low. We followed the same procedure for 10,000,000 samples and computed the relative frequency of the ranks, which are the ultimate the probabilities of the ranks of the tests by the simulation approach.

**b. Exact and Normal approximation approach.** For the CRW methods (both the exact and the normal approximate), we performed Monte Carlo (MC) simulations by considering the importance sampling approach. We considered 100,000 replications in the MC simulation to obtain smother probability curves. For the CRW method, we followed similar procedures regarding the parameters described in the simulation approach. In addition, we directly computed $F_0$ and $F_1$ from $F_0 = P(X_j > t) = \Phi(-t)$ and $F_1 = P(Y_l > t) = \Phi(\tau - t)$, respectively, to obtain the binomial probability of a test being higher than a specific test $t$.

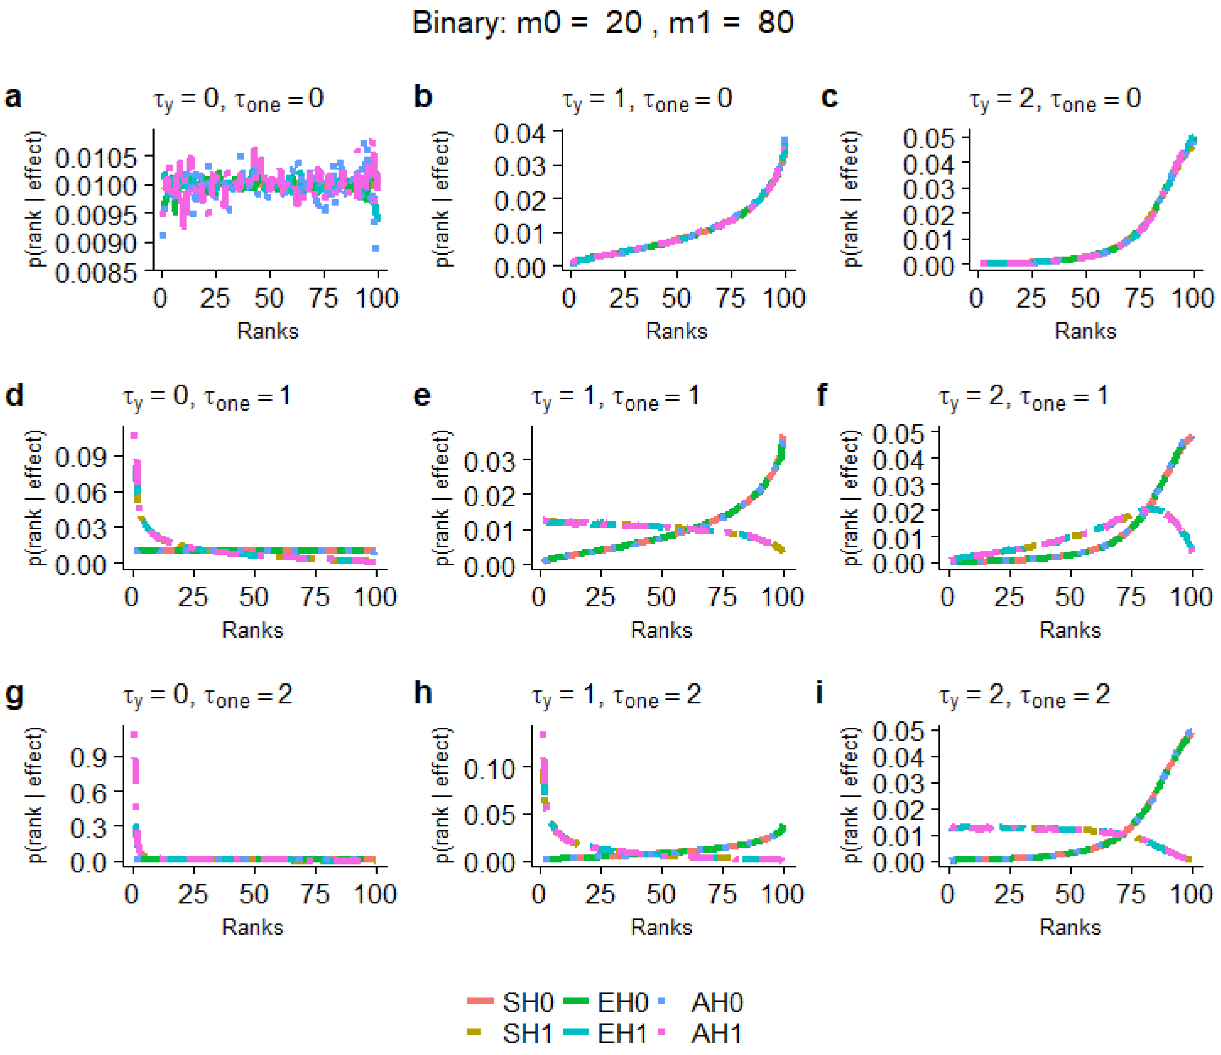


**Figure 7.2.1:** This figure shows $P(r_i = k|\tau_i)$ for the binary case in three different scenarios: 1) from the simulation, 2) from the exact CRW method, and 3) from the CRW normal approximation. To generate these plots, we assumed that there $m = 100$ tests of which $m_0 = 20$ are true nulls, and $m_1 = 80$ are true alternatives. Each plot consists of six curves, SH0, SH1, EH0, EH1, AH0, and AH1, where the first letter represents the method (S = simulated, E = exact, and A = approximate), and H0 and H1 represent the hypothesis type. Three curves (SH0, EH0, and AH0) starting from bottom-left represent $P(r_i = k|\tau_i = 0)$, and the remaining three curves (SH1, EH1, and AH1) starting from top-left represent $P(r_i = k|\tau_i = \tau_{one})$, where $\tau_{one} = \{0,1,2\}$. All the curves show the probability of the rank of the test with effect size either $\tau_i = 0$ or $\tau_i = \tau_{one}$ across all tests. For example, for the curve of the sixth plot (starting from left-right), there are 20 tests from the null models with effect size 0; 79 tests with effect size $\tau_y = 2$ and one test with the effect size $\tau_{one} = 1$ are from the alternative models. Thus, the curves SH1, EH1, and AH1 show the probability of the alternative test with effect size $\tau_{one} = 1$ being higher in rank than the other tests, and SH0, EH0, and AH0 show the probability of a null test with effect size 0 being higher in rank than the other tests. All plots of the simulation suggest nearly perfect alignment with the CRW (exact and approximate) methods.

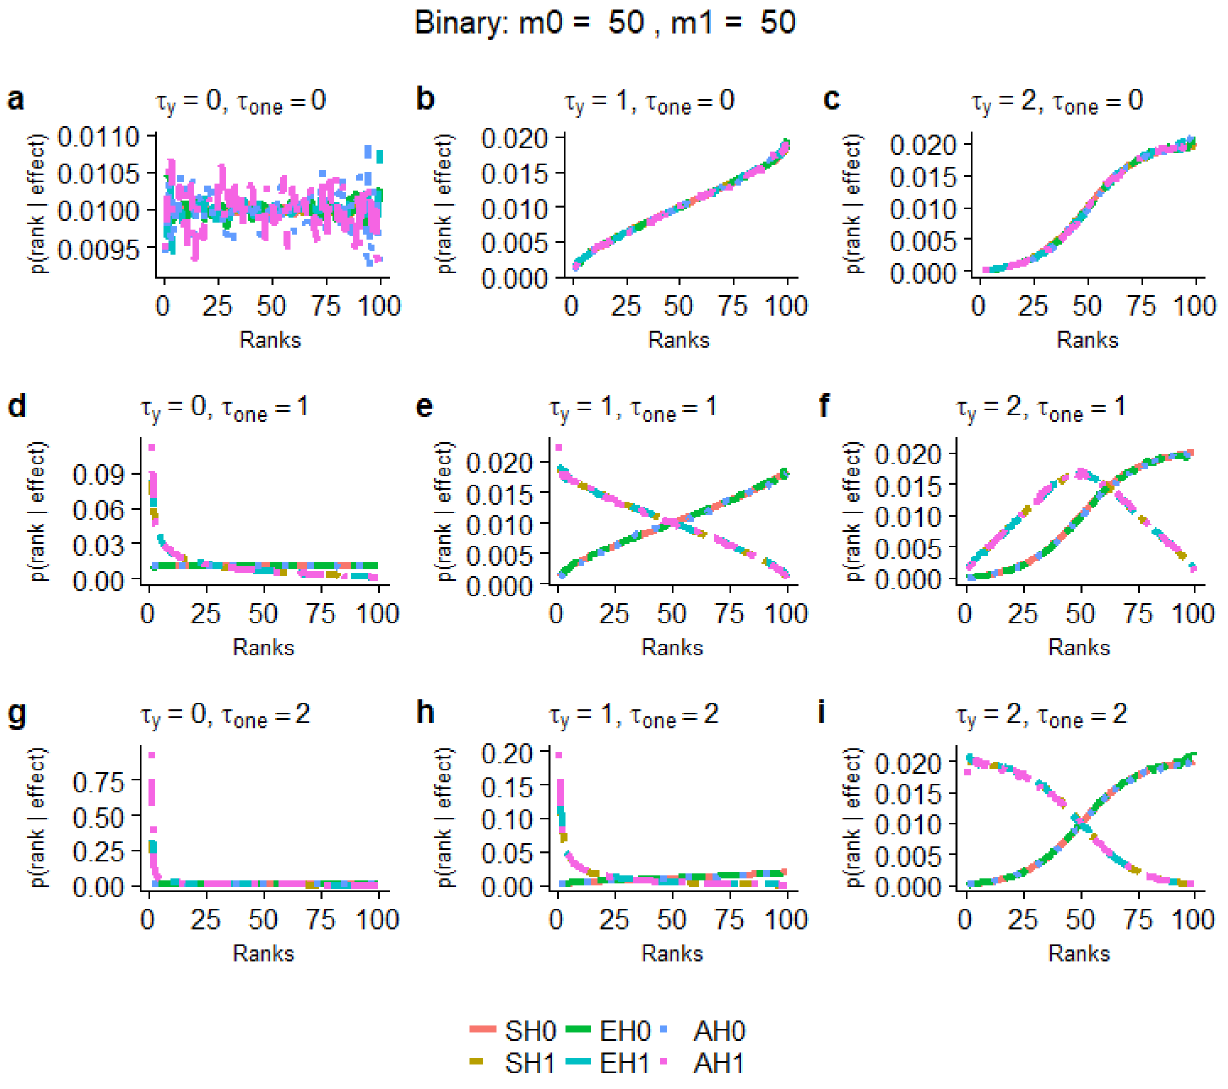


**Figure 7.2.2:** This figure shows $P(r_i = k|\tau_i)$ for the binary case in three different scenarios. To generate these plots, we assumed that there $m = 100$ tests of which $m_0 = 50$ are true nulls and $m_1 = 50$ are true alternatives.

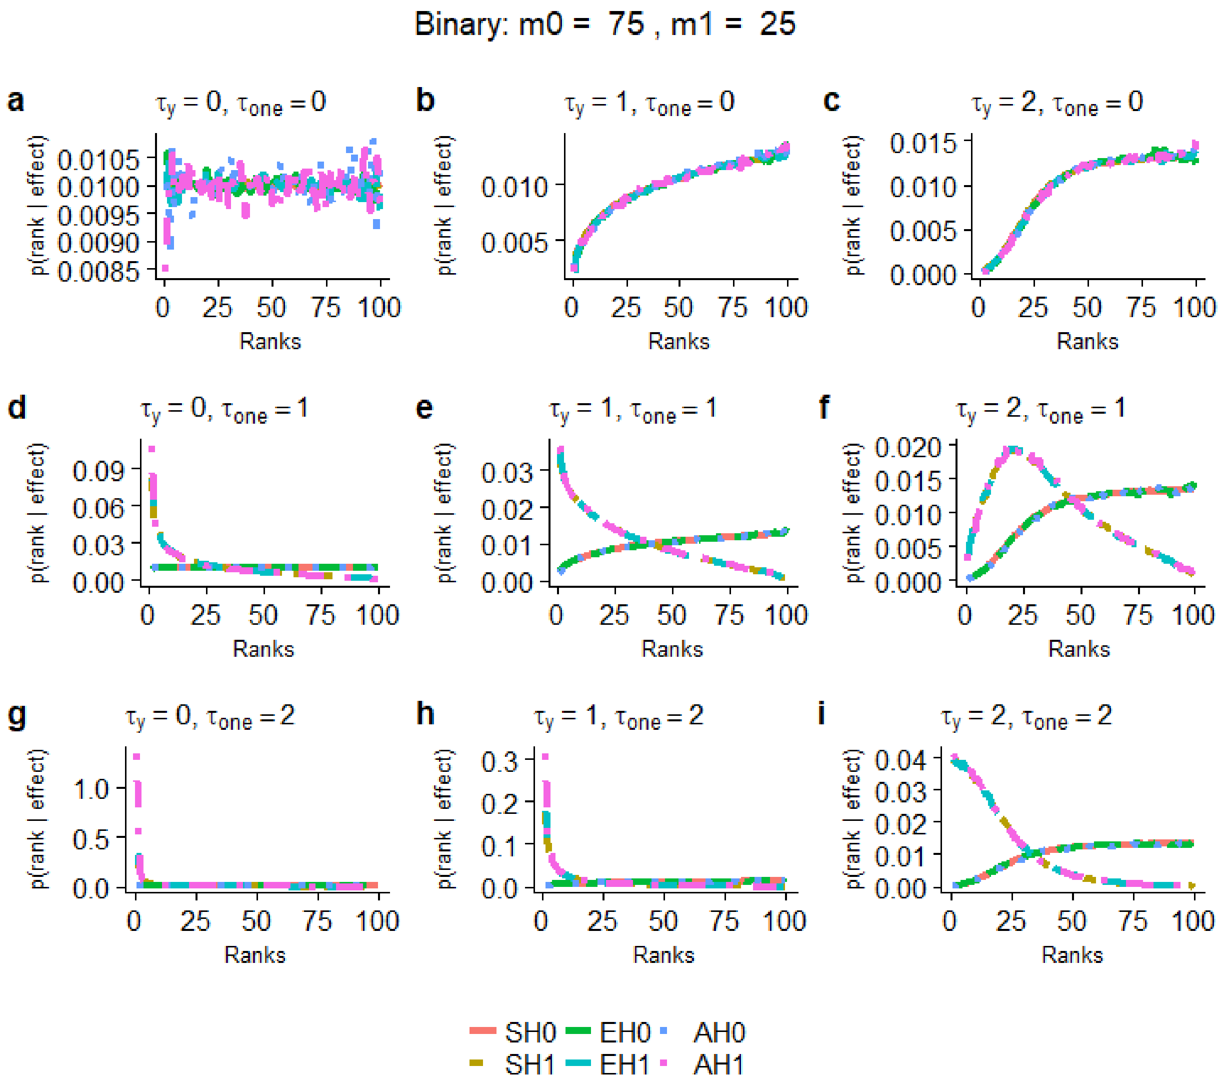


**Figure 7.2.3:** This figure shows $P(r_i = k|\tau_i)$ for the binary case in three different scenarios. To generate these plots, we assumed that there $m = 100$ tests of which $m_0 = 75$ are true nulls and $m_1 = 25$ are true alternatives.

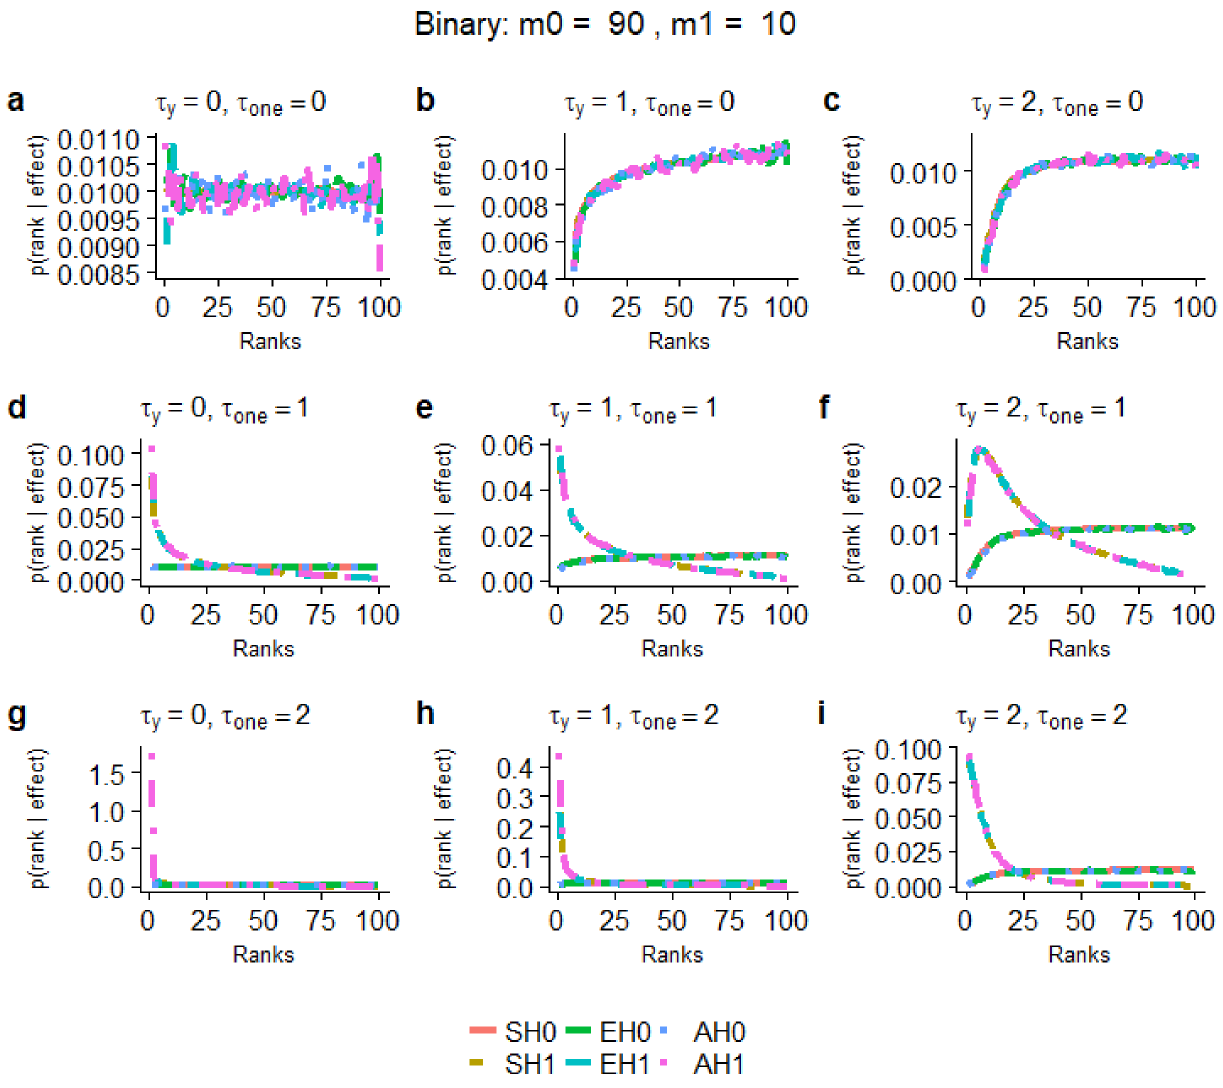


**Figure 7.2.4:** This figure shows $P(r_i = k|\tau_i)$ for the binary case in three different scenarios. To generate these plots, we assumed that there $m = 100$ tests of which $m_0 = 90$ are true nulls and $m_1 = 10$ are true alternatives.

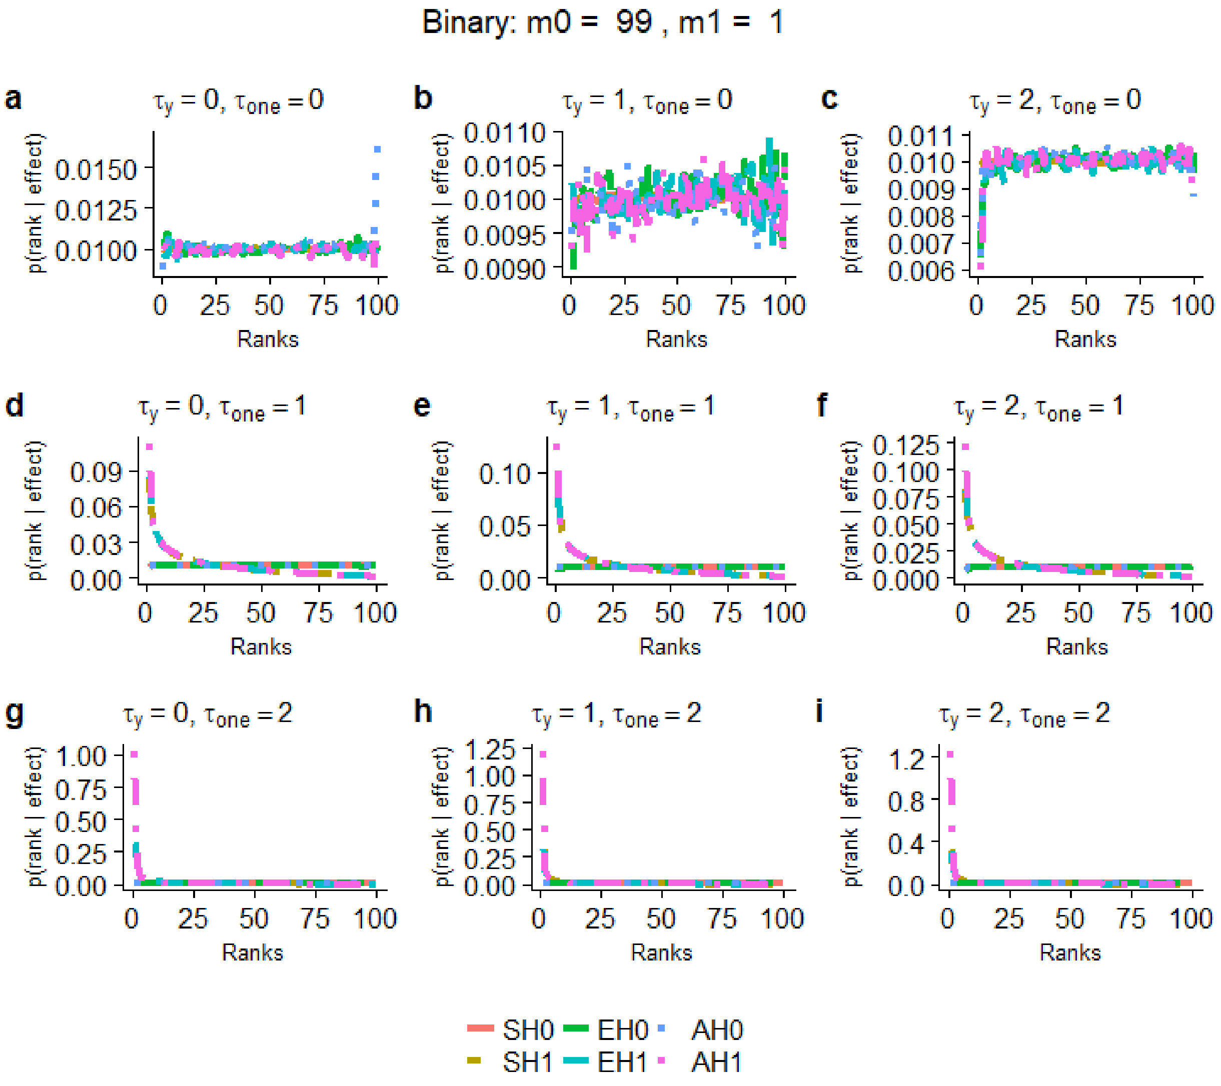


**Figure 7.2.5:** This figure shows $P(r_i = k|\tau_i)$ for the binary case in three different scenarios. To generate these plots, we assumed that there $m = 100$ tests of which $m_0 = 99$ are true nulls and $m_1 = 1$ are true alternatives.

## 8. Probability of ranks and weights.

This section shows the probabilities of the ranks given the mean covariate effect size, $P(r_i = k|E(\varepsilon_i))$, and the corresponding normalized weights, $w_i$, versus the ranks.

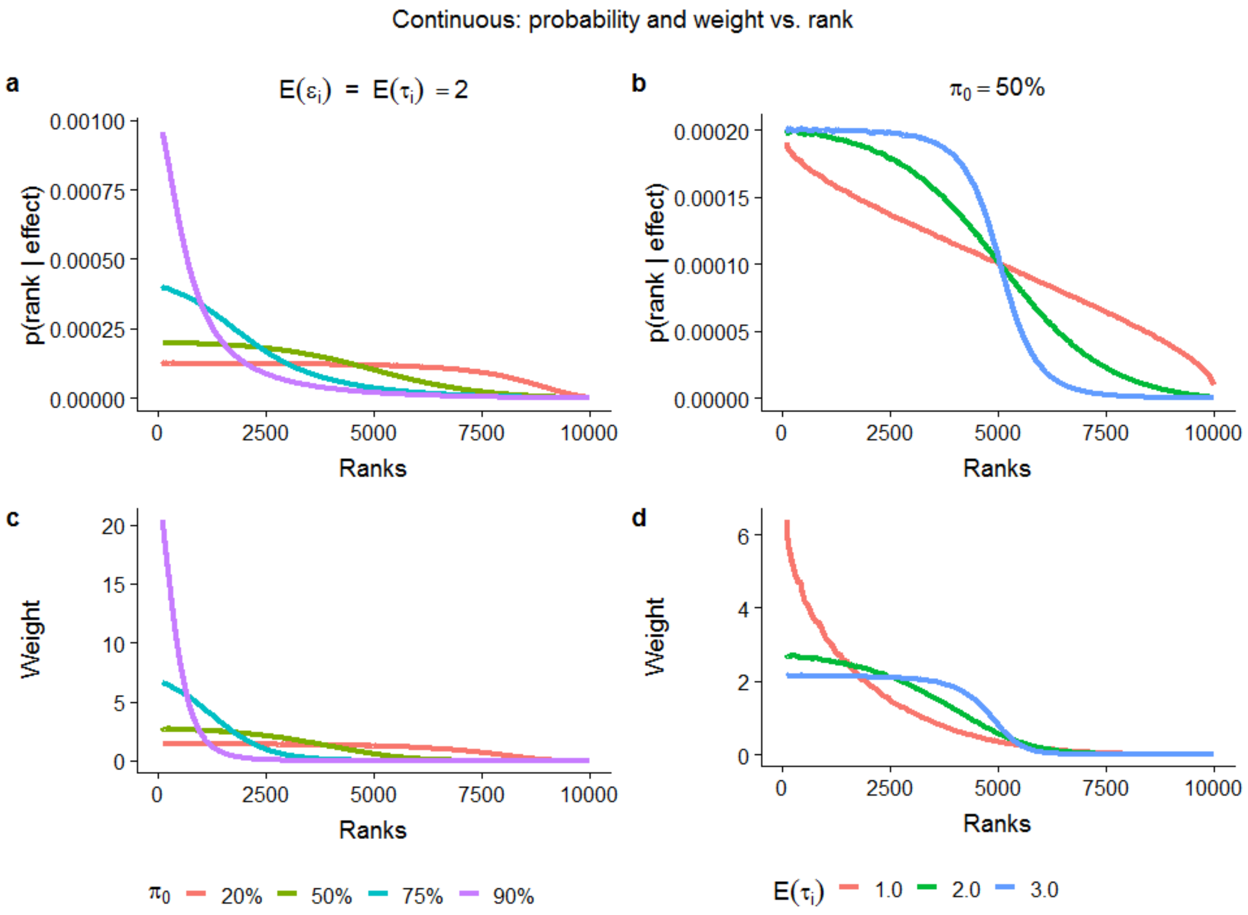


**Figure 8.1:** This Figure shows the probabilities, $P(r_i = k|E(\varepsilon_i))$, and the corresponding normalized weights, $w_i$, versus ranks for the continuous case, where the mean covariate effect size $E(\tau_i) = E(\varepsilon_i)$. The first column is for the different proportion of the true null hypothesis when the mean test effect and the mean covariate effect sizes are the same, and the second colum is for the different effect sizes when the proportion of the true null tests is 50%. To generate this plot, we applied the CRW normal approximation method. We assumed that there are $m = 10{,}000$ hypotheses tests; the test statistics follow normal distributions with mean 0 and $\varepsilon_i$ under the null and alternative hypothesis, respectively, and standard deviations 1.

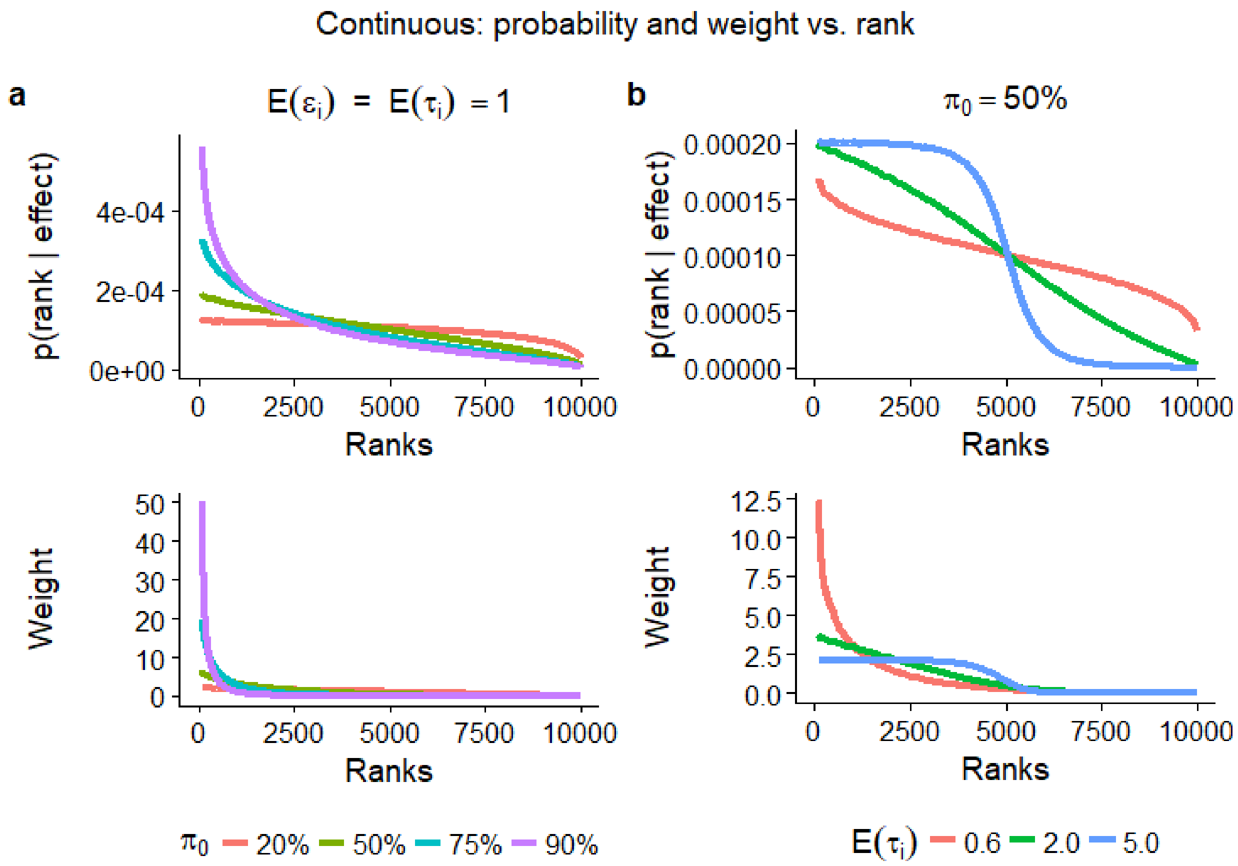


**Figure 8.2:** This Figure shows the probabilities, $P(r_i = k|E(\varepsilon_i))$, and the corresponding normalized weights, $w_i$, versus ranks for the continuous case.

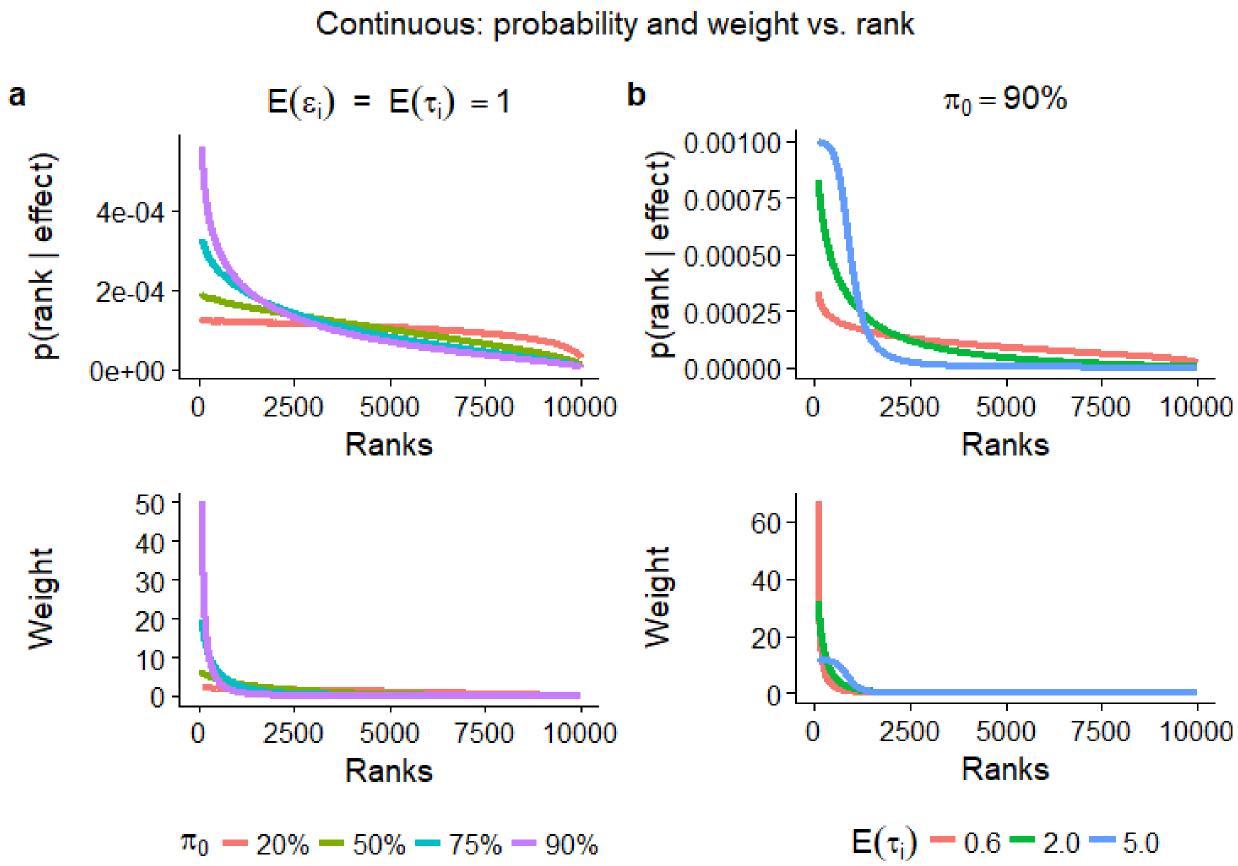


**Figure 8.3:** This Figure shows the probabilities, $P(r_i = k|E(\varepsilon_i))$, and the corresponding normalized weights, $w_i$, versus ranks for the continuous case.

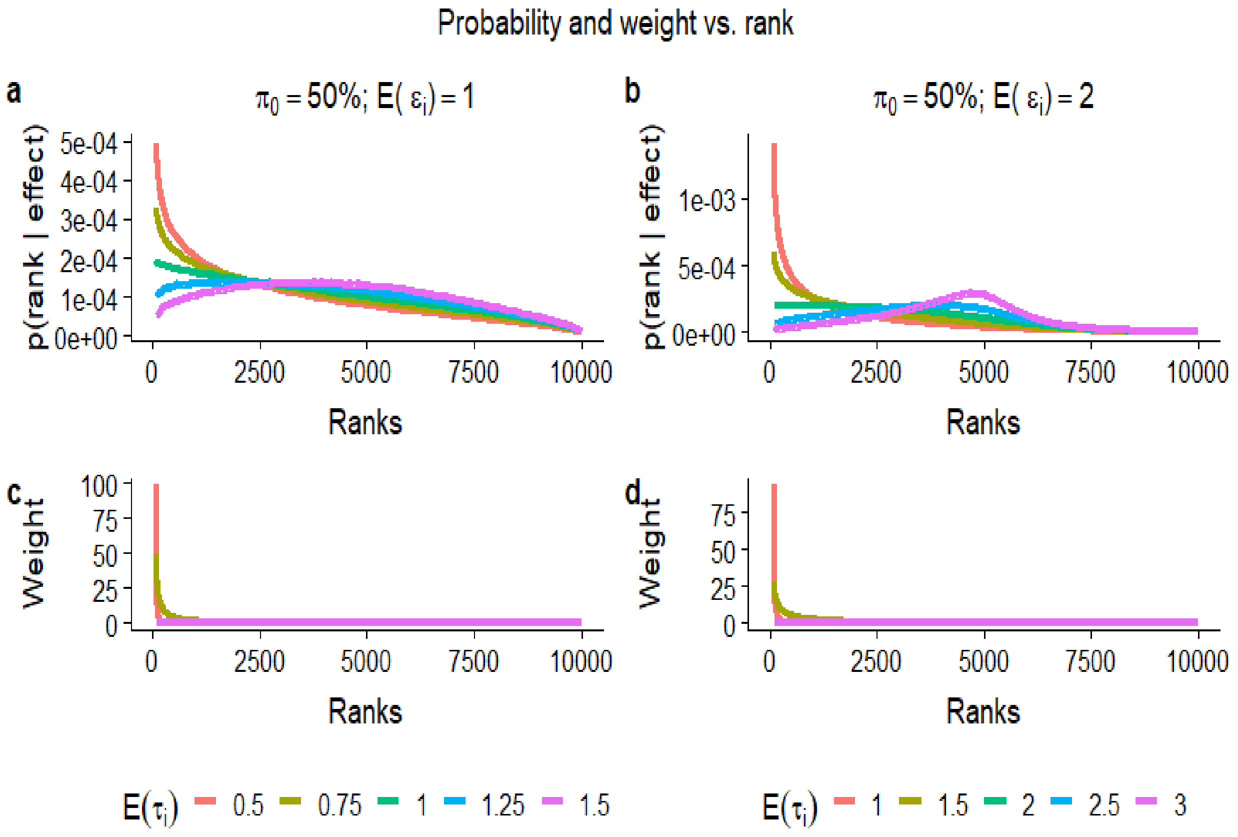


**Figure 8.4.** This figure shows rank probability and weights when the test effect and covariate effect are not equal. The test effect is one in the left column and two in the right column. The different curves correspond to covariate effects as shown. There were 50% null tests in these plots.

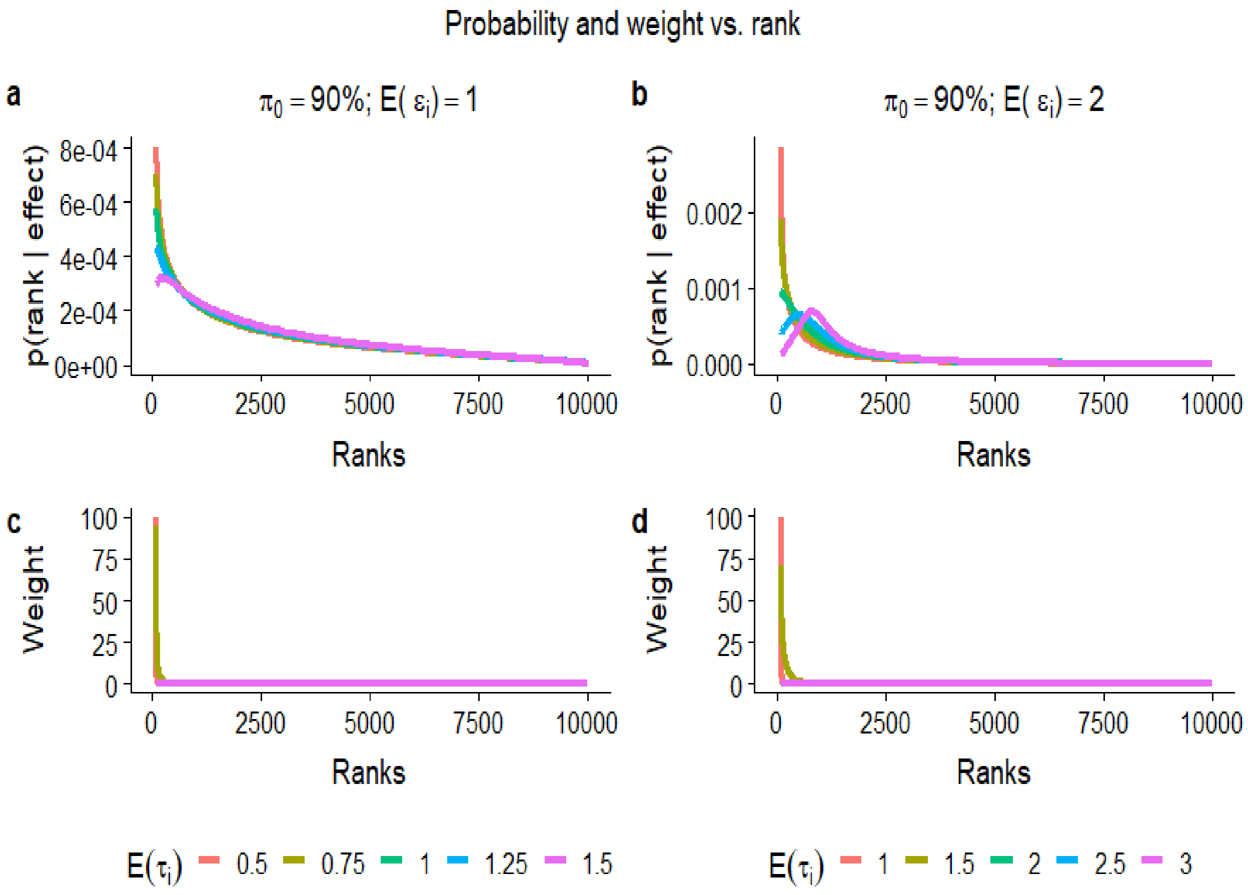


**Figure 8.5.** This figure shows rank probability and weights when the test effect and covariate effect are not equal. The test effect is one in the left column and two in the right column. The different curves correspond to covariate effects as shown. There were 90% null tests in these plots.

## 9. Family-wise error rate (FWER).

### 9.1. FWER when all tests are from true null models.

We conducted simulations to verify that the CRW method controls the Family Wise Error Rate (FWER). For the simulation, we performed 1,000 replications, and for each replication, we generated a data set composed of $m = 10{,}000$ observations of three variables: 1) test statistics, 2) p-values of the two-tailed tests, and 3) covariate statistics. We generated test and covariate statistics from the standard normal distribution, and p-values were computed from the test statistics using z-score criteria. Then we performed simple regression to obtain a relationship between the test and covariate statistics in which covariate statistics were regressed on the test statistics. We computed predicted covariate statistics for the mean and median test statistics and used the predicted values as the estimate of the covariate effect size for the continuous and binary cases, respectively. We then applied the predicted covariate statistic to compute the probability of the rank and the corresponding mean test statistic to compute the weight for the continuous case. Similarly, we used the predicted covariate statistic and corresponding median test statistic to compute the probability and the weight for the binary case, respectively. At the end, we compared the sorted p-values with the weighted significance thresholds and then computed the proportion of the rejected null hypothesis to obtain the FWER. Since all test statistics are generated from the null models, we would expect the number of false positive to be below the significance level of $\alpha$. From Figure 9.1.1, we see the CRW methods control the FWER and perform similarly to the Bonferroni correction.

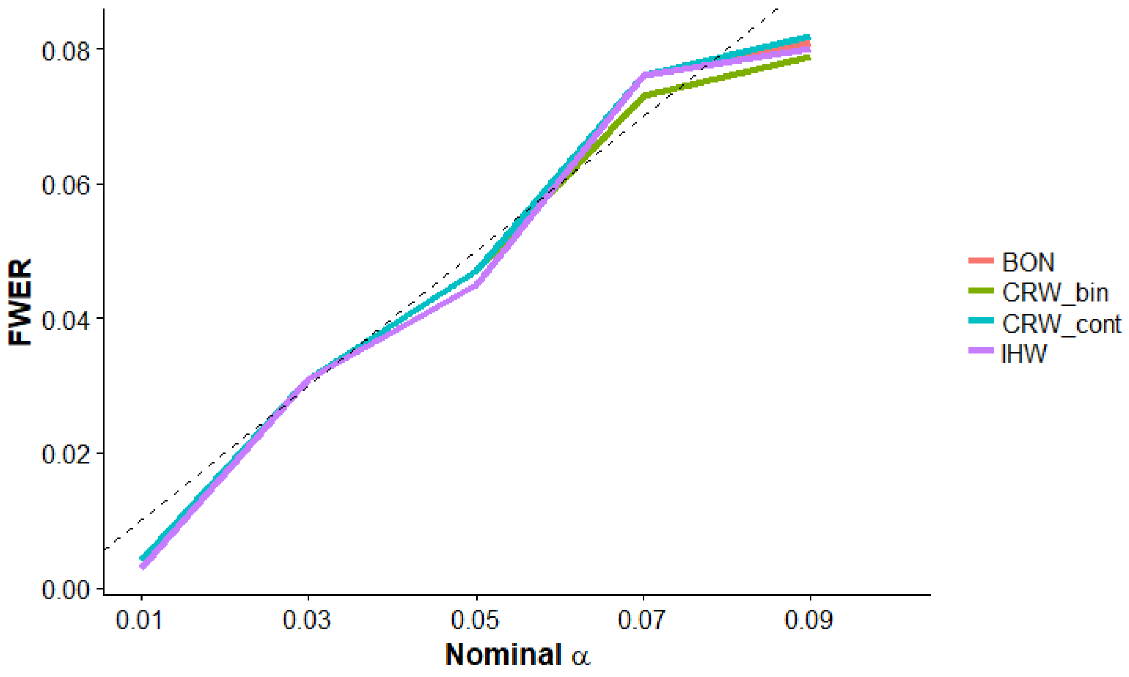


**Figure 9.1.1:** This Figure shows the FWER for different significance levels of $\alpha$. In the legend, the representation is: BON = Bonferroni, CRW_bin = CRW binary, CRW_cont = CRW continuous, and IHW = Independent Hypothesis Weighting. To generate these plots, we performed 1,000 replications of $m = 10{,}000$ hypothesis tests. Consequently, to obtain the FWER, the test statistics of the hypothesis tests were generated from the standard normal distribution and then the proportion of the rejected null hypothesis was computed.

## 9.2. FWER for different effect sizes.

### 9.2.1. Continuous effects.

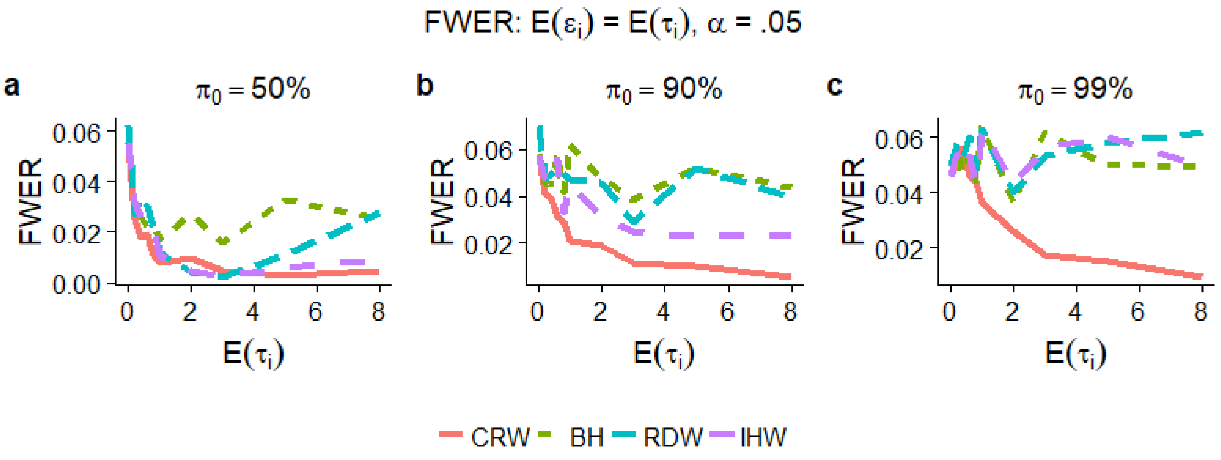


**Figure 9.2.1.1:** This Figure shows the simulated FWER for different mean effect sizes when the mean test effect $E(\varepsilon_i)$ is equal to mean covariate effect $E(\tau_i)$. Three columns are based on three groups composed of $50\%, 90\%$, and $99\%$ true null hypothesis. To generate these plots, we conducted 1,000 replications and assumed that there were 10,000 hypotheses tests.

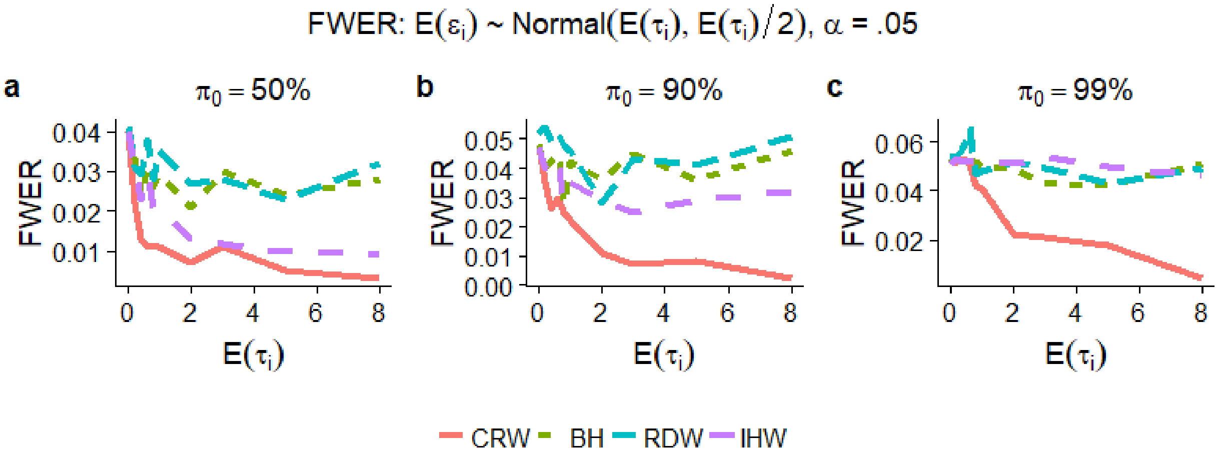


**Figure 9.2.1.2:** This Figure shows the simulated FWER when the mean test effect $E(\varepsilon_i)$ is not equal to mean covariate effect $E(\tau_i)$; rather $E(\varepsilon_i) \sim Normal(E(\tau_i), \frac{E(\tau_i)}{2})$.

## 9.2.2. Binary effects.

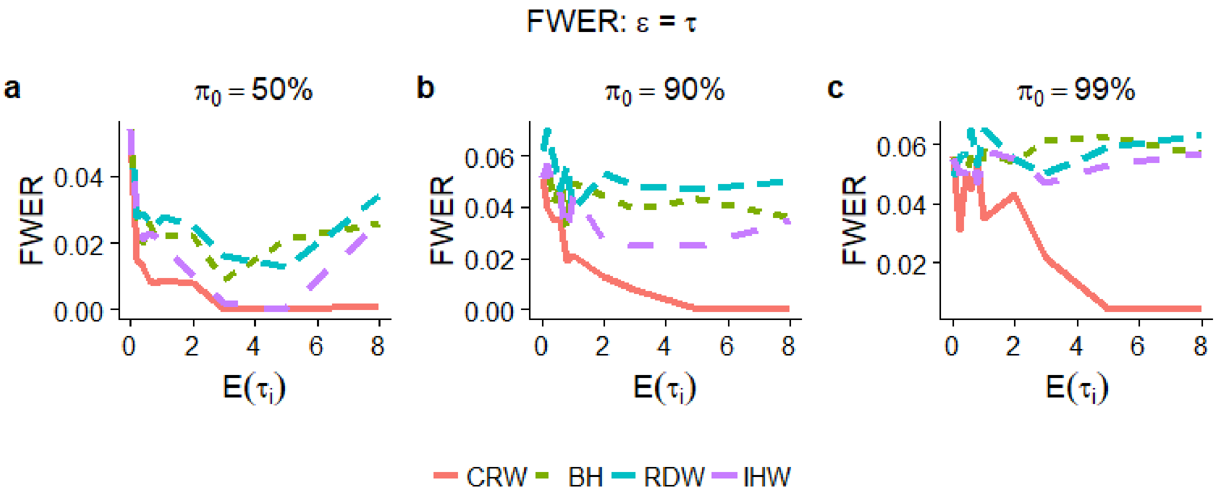


**Figure 9.2.2.1:** This Figure shows the simulated FWER for different effect sizes when the common test effect $\varepsilon$ is equal to common covariate effect $\tau$.

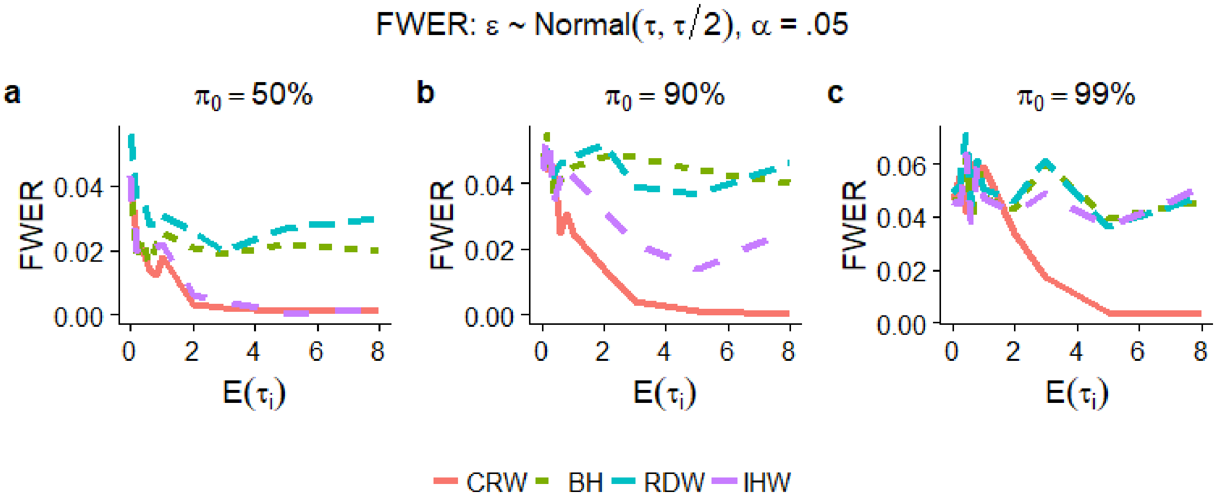


**Figure 9.2.2.2:** This Figure shows the simulated FWER when the common alternative test effect $\varepsilon$ is not equal to the common covariate effect $\tau$; rather $\varepsilon \sim Normal(\tau, \frac{\tau}{2})$.

## 10. False discovery rate (FDR).

### 10.1. Continuous effects.

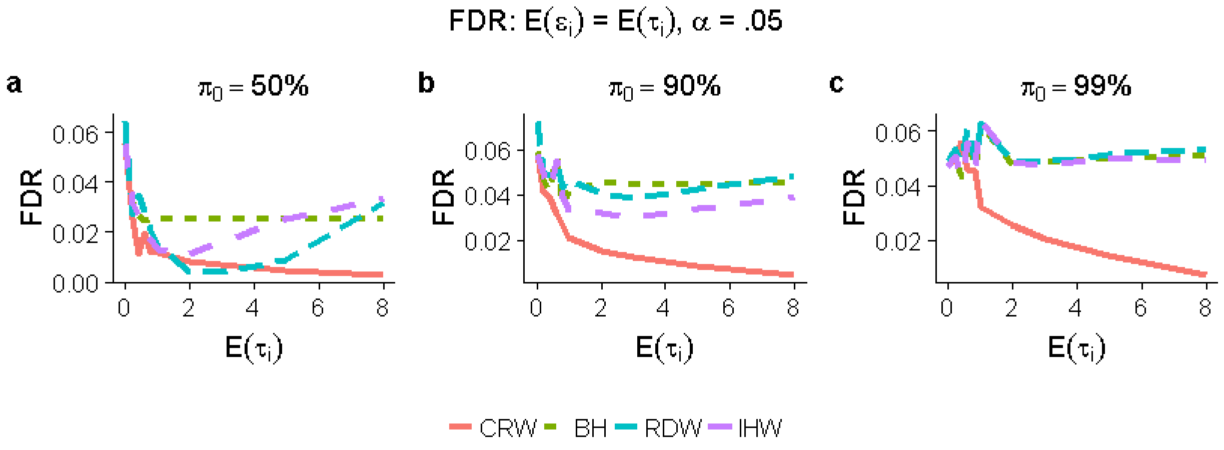


**Figure 10.1.1:** This Figure shows the simulated FDR for different mean effect sizes when the mean test effect $E(\varepsilon_i)$ is equal to mean covariate effect $E(\tau_i)$. Three columns are based on three groups composed of 50%, 90%, and 99% true null hypothesis. To generate these plots, we conducted 1,000 replications and assumed that there were 10,000 hypotheses tests.

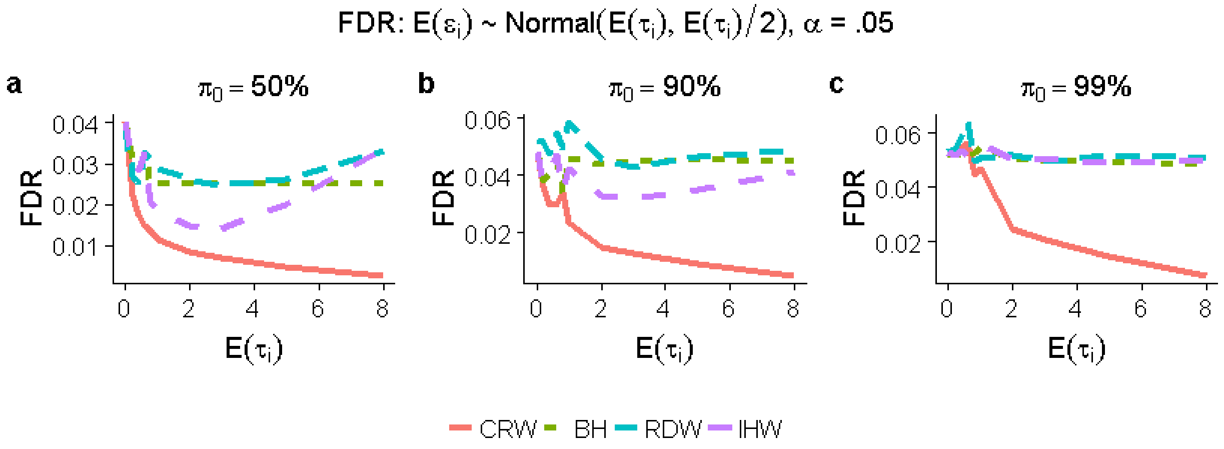


**Figure 10.1.2:** This Figure shows the simulated FWER when the mean test effect $E(\varepsilon_i)$ is not equal to mean covariate effect $E(\tau_i)$; rather $E(\varepsilon_i) \sim Normal(E(\tau_i), \frac{E(\tau_i)}{2})$.

## 10.2. Binary effects.

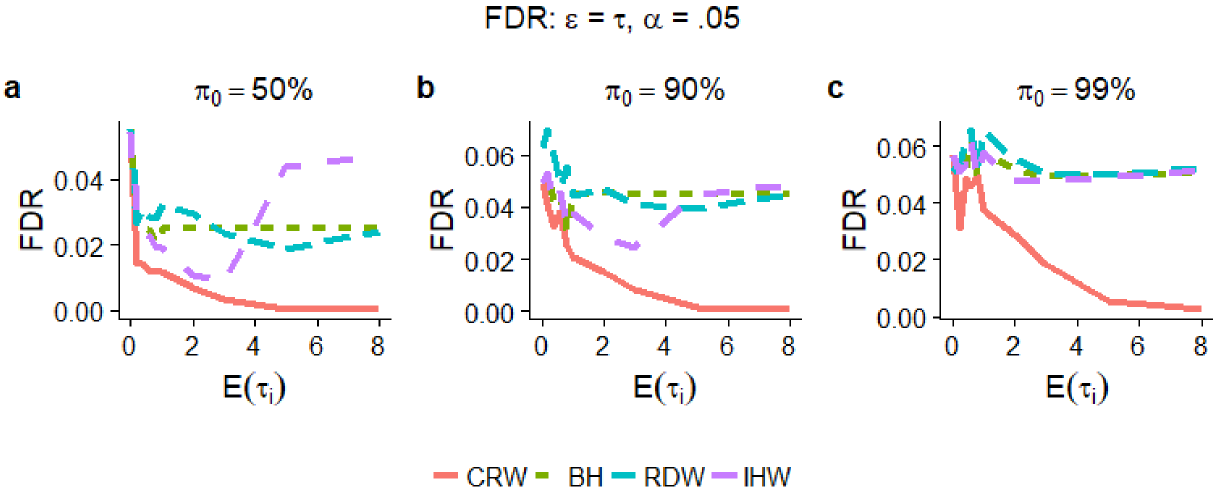


**Figure 10.2.1:** This Figure shows the simulated FDR for different effect sizes when the common test effect $\varepsilon$ is equal to common covariate effect $\tau$.

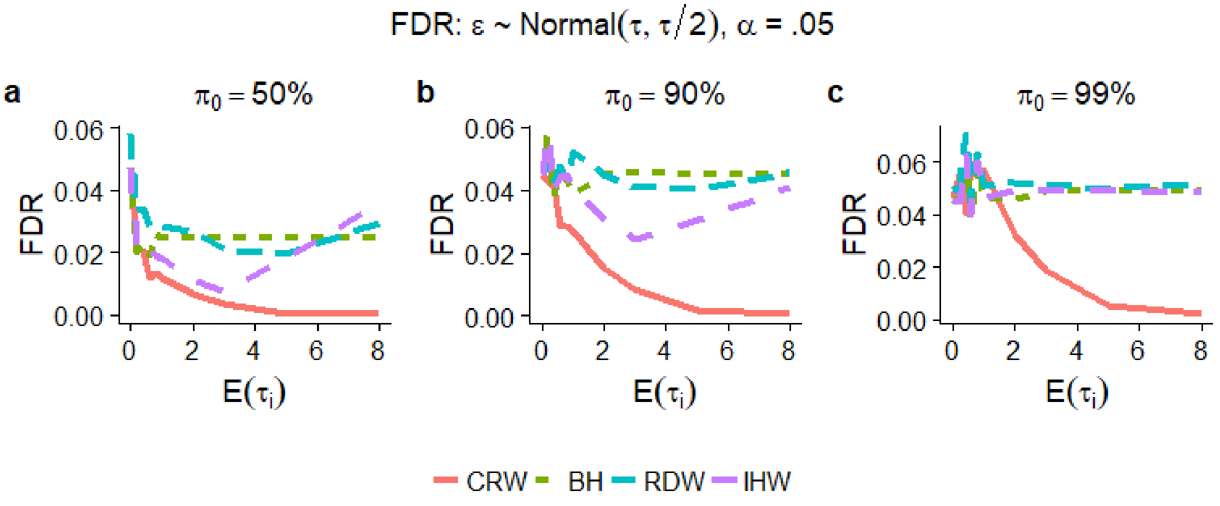


**Figure 10.2.2:** This Figure shows the simulated FDR when the common alternative test effect $\varepsilon$ is not equal to the common covariate effect $\tau$; rather $\varepsilon \sim Normal(\tau,\ \frac{\tau}{2})$.

**11. Power vs. effect size.**

**11.1. Continuous effects.**

See the original article.

**11.2. Binary effects.**

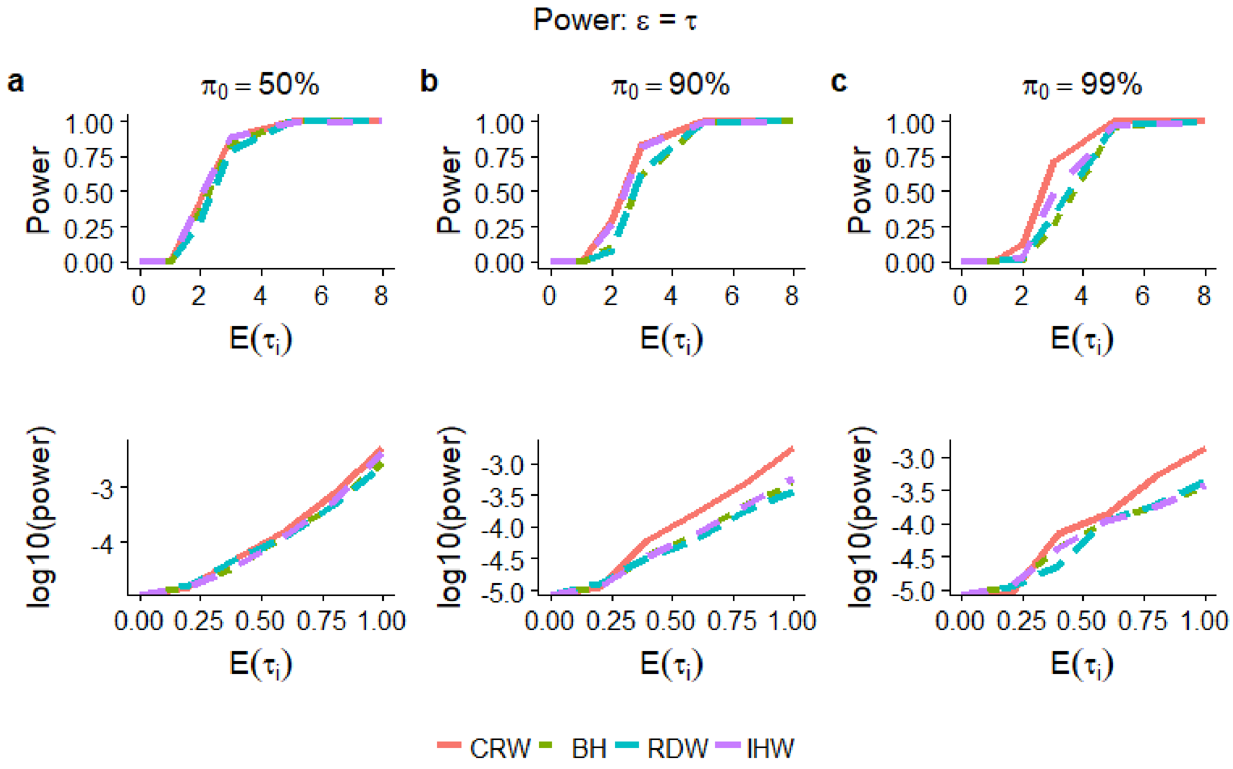


**Figure 11.2.1:** This Figure shows the simulated Power for the different effect sizes when the common alternative test effect $\varepsilon$ is equal to covariate effect $\tau$. Each plot consists of four curves based on CRW, Benjamini-Hochberg (BH), Roeder and Wasserman (RDW), and Independent Hypothesis Weighting (IHW) methods. The first row shows the power for low to high effect sizes, and the second row shows power for the low effect sizes. Three columns are based on three groups composed of 50%, 90%, and 99% true null hypothesis. To generate these plots, we conducted 1,000 replications and assumed that there were 10,000 hypotheses tests. For each replication, we average Power then calculated the average across the replications.

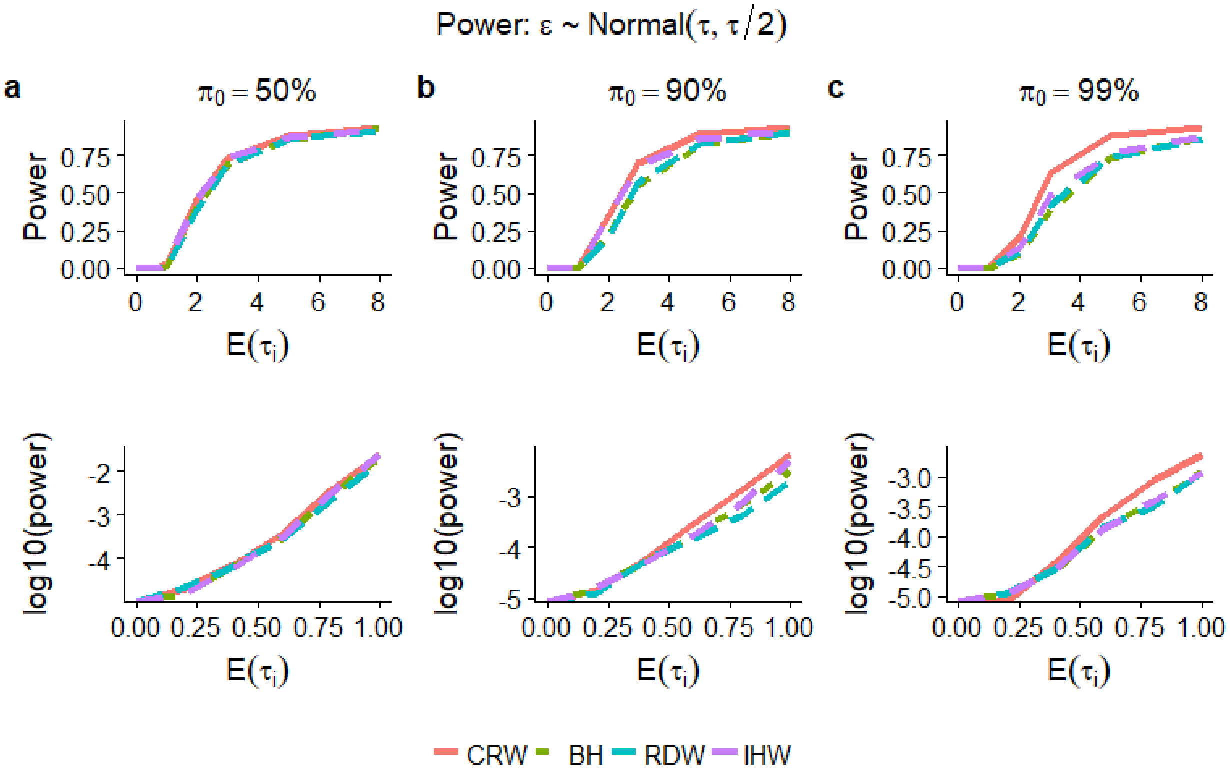


**Figure 11.2.2:** This Figure shows the simulated Power for the binary effect sizes when the common alternative test effect $\varepsilon$ is not equal to the covariate effect $\tau$; rather $\varepsilon \sim Normal(\tau,\ \frac{\tau}{2})$.

## 12. Power vs. variance of test effect.

This section shows the influence of the variance of the mean test effect size $E(\varepsilon_i)$ across different mean covariate effect sizes $E(\tau_i)$.

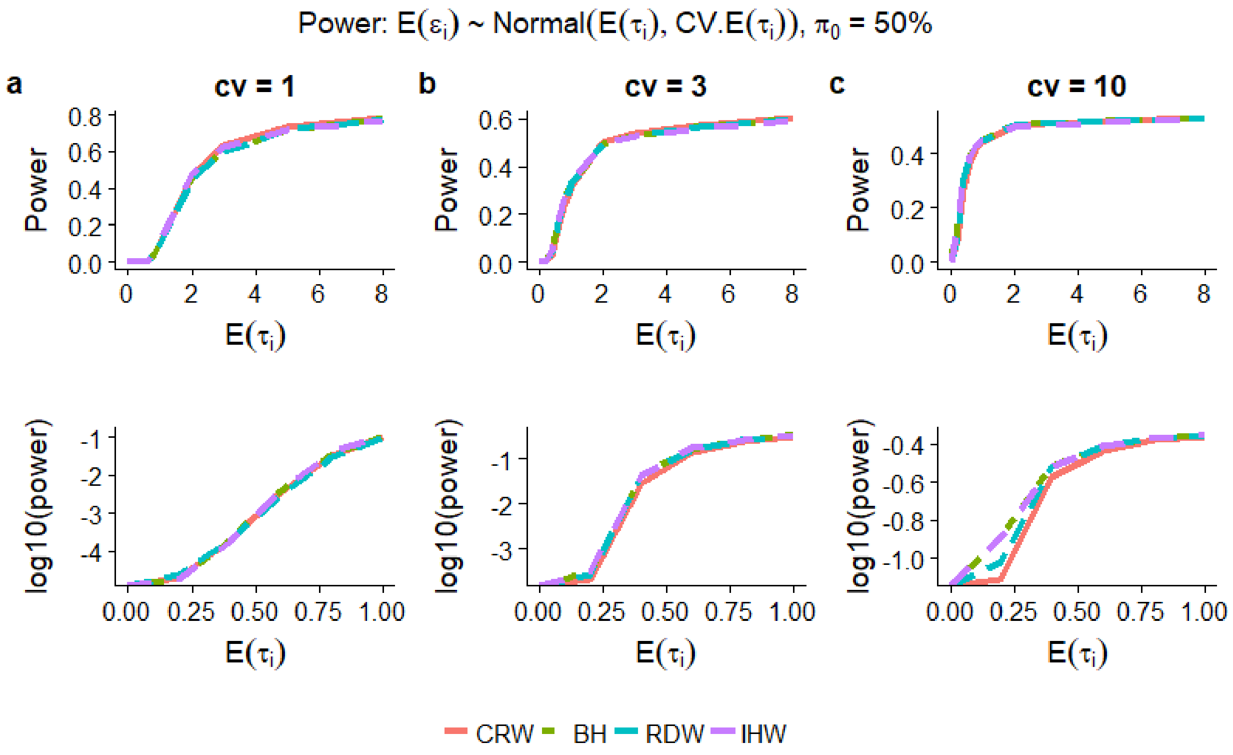


**Figure 12.1:** The simulated Power when the mean test effect $E(\varepsilon_i)$ is not equal to mean covariate effect $E(\tau_i)$; rather $E(\varepsilon_i) \sim Normal(E(\tau_i), CV.E(\tau_i))$, where CV = coefficient of variations. Each plot consists of four curves based on CRW, Benjamini-Hochberg (BH), Roeder and Wasserman (RDW), and Independent Hypothesis Weighting (IHW) methods. The first row shows the power for low to high effect sizes, and the second row shows power for the low effect sizes. Three columns are based on three groups composed of $CV = 1$, 3, or 10 true null hypotheses. To generate these plots, we conducted 1,000 replications and assumed that there were 10,000 hypotheses tests of which 50% are from the true null models. For each replication, we average Power then calculated the average across the replications

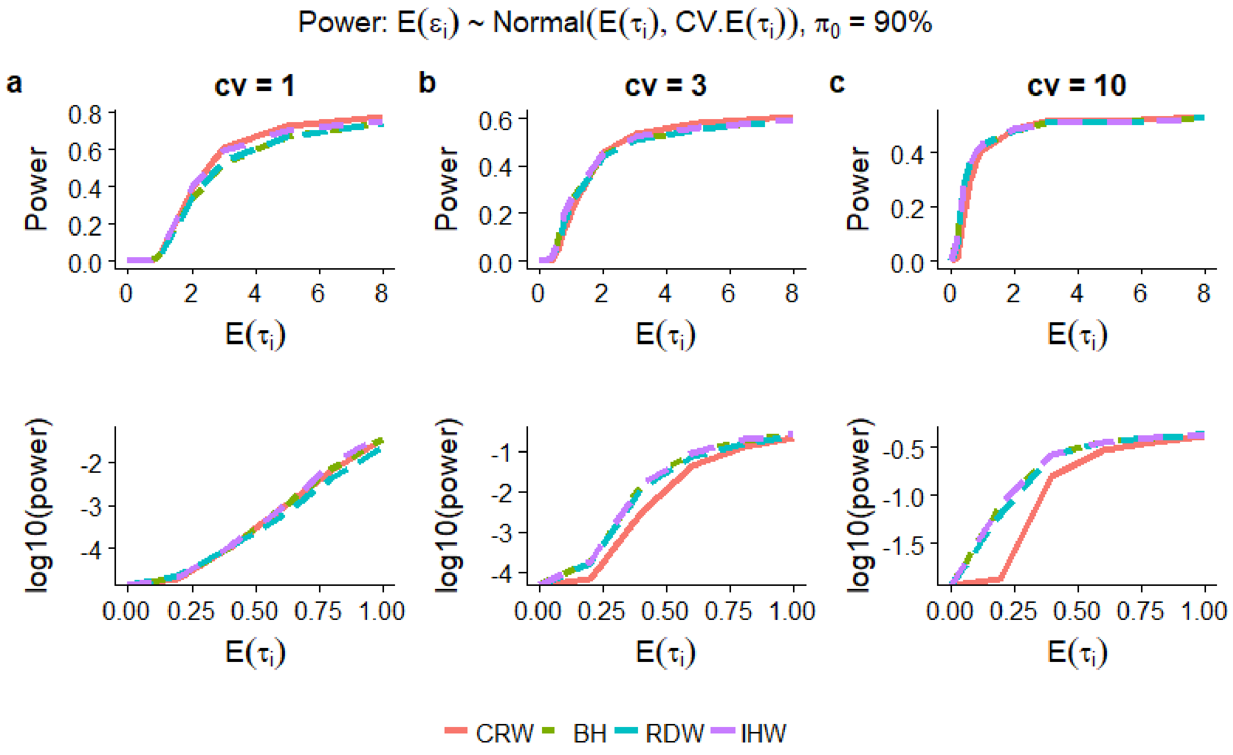


**Figure 12.2:** This Figure shows the simulated FWER when the mean test effect $E(\varepsilon_i)$ is not equal to mean covariate effect $E(\tau_i)$; rather $E(\varepsilon_i) \sim Normal(E(\tau_i),\ CV.E(\tau_i)$, where CV = coefficient of variations. To generate these plots, we conducted 1,000 replications and assumed that there were 10,000 hypotheses tests of which 90% are from the true null models.

**13. Power vs. proportion of true null hypothesis.**

The CRW method performs well when the proportion of the true alternatives are low, especially when it is below 20%. Generally, in the multiple hypothesis settings, this is the actual scenario in which only a fraction of the tests is from the true alternatives. Our method does not affect by the null proportion if the mean covariate effect size $E(\tau_i)$ and the correlation between the test statistics are low. For the moderate mean effect size and the high correlation, our method performs better as long as the proportion of the true null test is above 60%. In addition; the CRW method always performs well if the null proportion is high, approximately above 80%, regardless of the test correlations and mean covariate effect sizes.

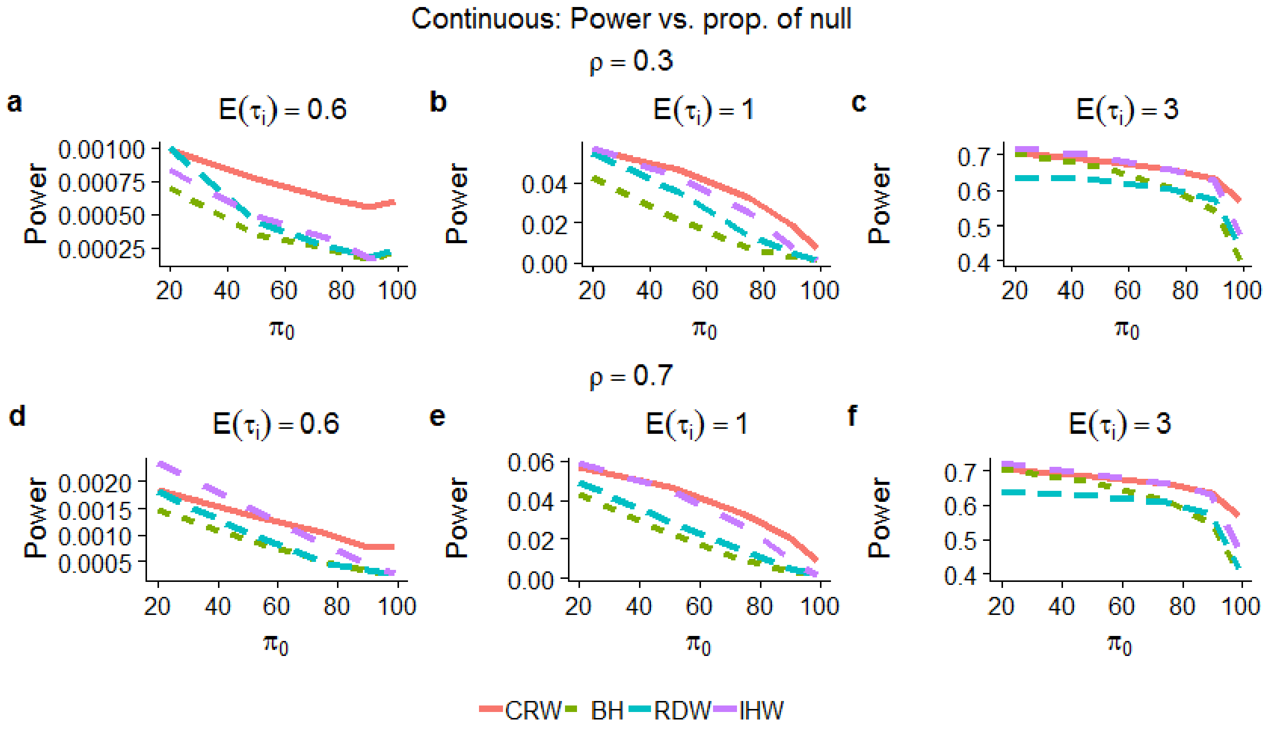


**Figure 13.1:** This Figure shows the simulated power across the proportion of the true null hypothesis for the different test correlations for the continuous effects. To generate these plots, we assumed that there were $m = 10{,}000$ hypotheses. We also assumed that the mean test effect size $E(\varepsilon_i)$ and the mean covariate effect size $E(\tau_i)$ are the same.

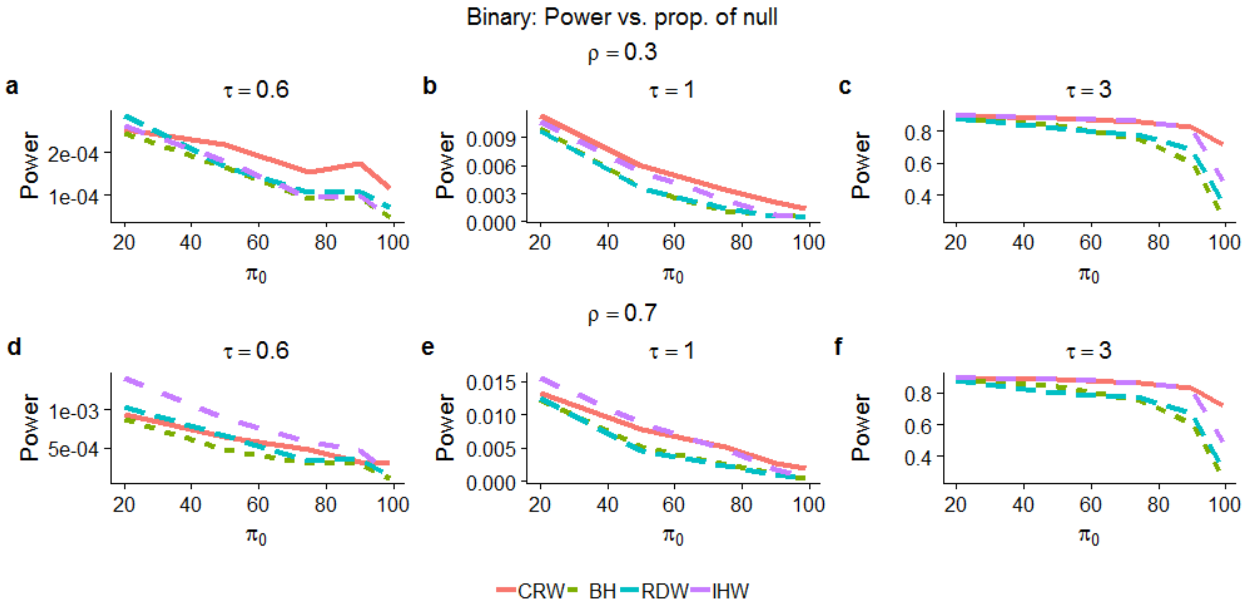


**Figure 13.2:** This Figure shows the simulated power across the proportion of the true null hypothesis for the different test correlations for the binary effects. To generate these plots, we assumed that there were $m = 10{,}000$ hypotheses. We also assumed that the common test effect size $\varepsilon$ and the common covariate effect size $\tau$ are the same.

## 14. Power vs. test correlation.

As mentioned earlier, our CRW method does not affect by the null proportion if the mean covariate effect size $E(\tau_i)$ and the correlation between the test statistics are low. For the low mean effect size and the high correlation, our method performs better as long as the proportion of the true null test is above 60%. In addition; the CRW method always performs well if the null proportion is high, approximately above 80%, regardless of the test correlations and mean covariate effect sizes.

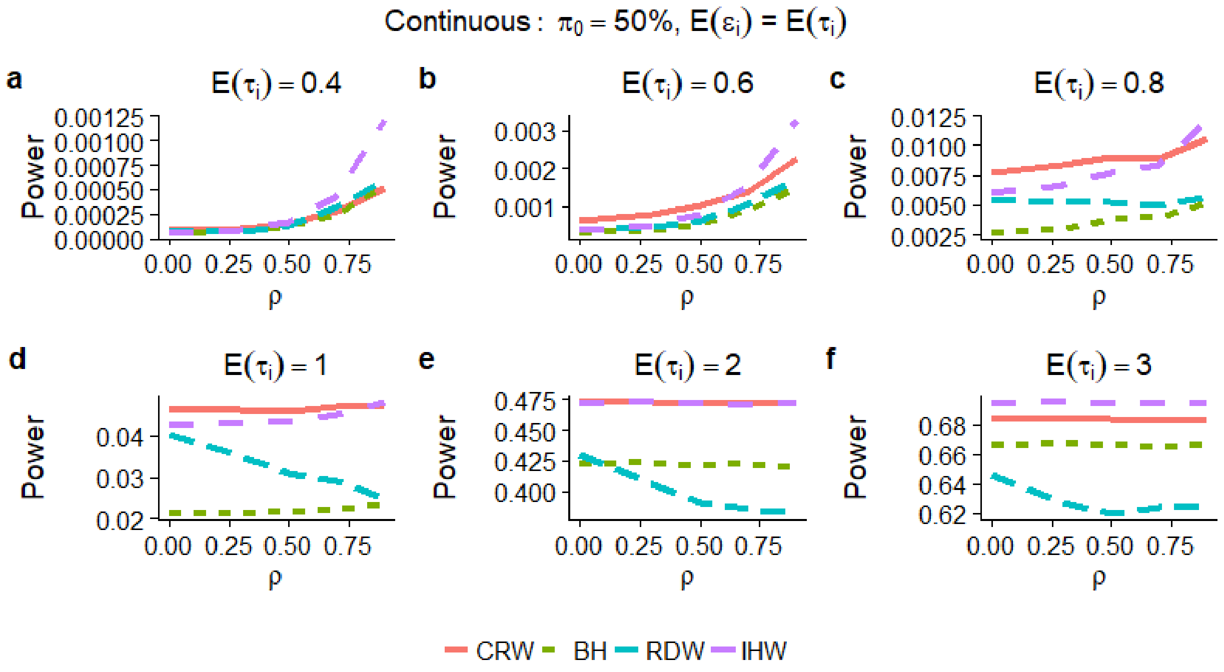


**Figure 14.1:** This Figure shows the simulated power across different correlations between the test statistics for various effect sizes. Each plot consists of four curves based on CRW, Benjamini-Hochberg (BH), Roeder and Wasserman (RDW), and Independent Hypothesis Weighting (IHW) methods. To generate these plots, we assumed that there were 10,000 hypotheses and of which 50% are true null. We also assumed that the mean test effect size $E(\varepsilon_i)$ and the mean covariate effect size $E(\tau_i)$ are the same.

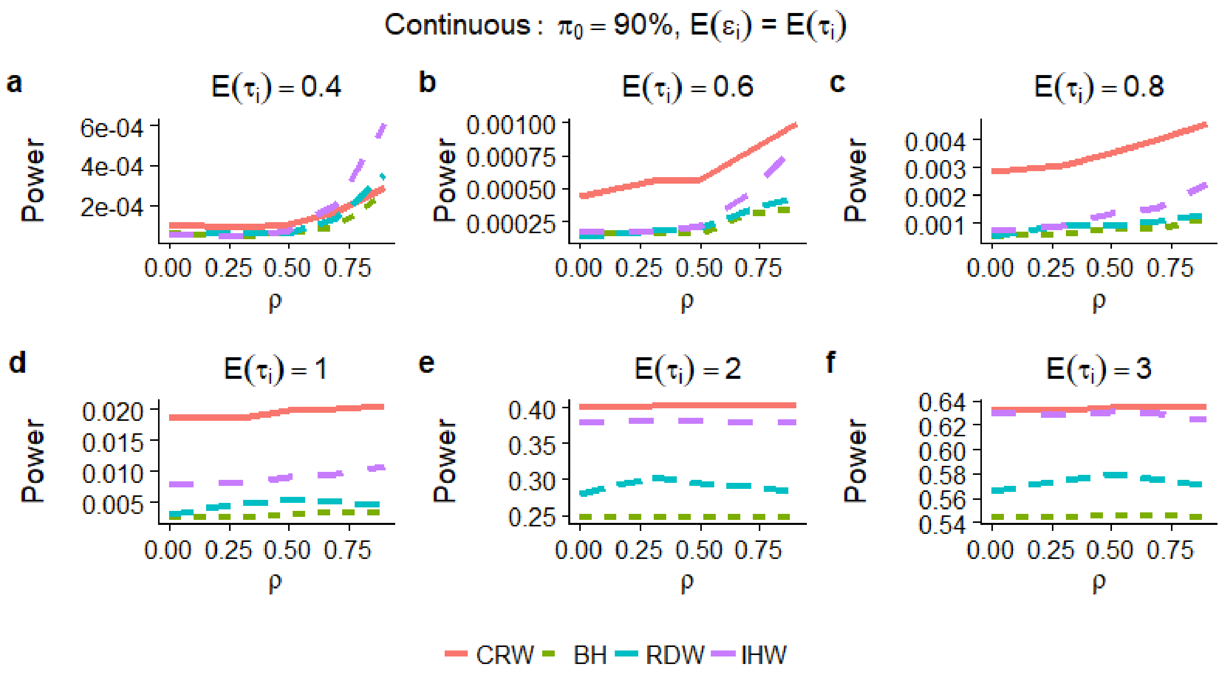


**Figure 14.2:** This Figure shows the simulated power across different correlations between the test statistics for various effect sizes. To generate these plots, we assumed that there were 10,000 hypotheses and of which 90% are true null.

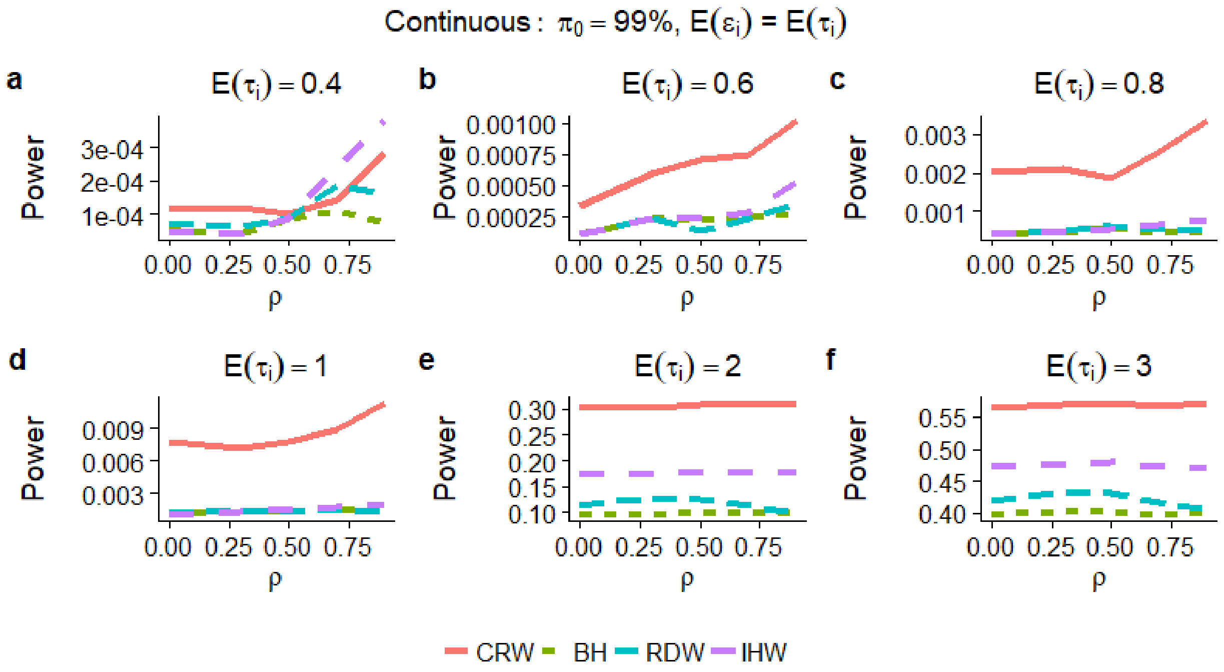


**Figure 14.3:** This Figure shows the simulated power across different correlations between the test statistics for various effect sizes when there were 10,000 hypotheses and of which 99% are true null.

**15. Relationship between covariate effect and test effect.**

The information in covariate rank weight method comes from the relationship between the test effect and the covariate effect. The covariate rank depends on the covariate effect size. If there is a high correlation between covariate effect and test effect, then the covariate rank will tend to be high when the test effect is high. We wanted to explore this relationship further. Let us suppose $\varepsilon_y$ is the covariate effect and the corresponding rank is $r_y$, and $\varepsilon_t$ is the test effect, Then the relationship between the probability of the rank given the test effect can be defined in terms of the probability of the rank given the covariate effect. If the effects are assumed continuous, then the relationship can be expressed as

$$P\left(r_y = k \middle| \varepsilon_t\right) = \frac{P\left(r_y,\ \varepsilon_t\right)}{P(\varepsilon_t)} = \int \frac{P\left(r_y,\ \varepsilon_y, \varepsilon_t\right) d\varepsilon_y}{P(\varepsilon_t)} = \int P\left(r_y \middle| \varepsilon_y, \varepsilon_t\right) P\left(\varepsilon_y \middle| \varepsilon_t\right) d\varepsilon_y.$$

Since including $\varepsilon_t$ does not add further information once the rank is computed from $\varepsilon_y$, the above expression becomes

$$P\left(r_y = k \middle| \varepsilon_t\right) = \int P\left(r_y \middle| \varepsilon_y\right) P\left(\varepsilon_y \middle| \varepsilon_t\right) d\varepsilon_y = E_{\varepsilon_y}\left(P\left(r_y \middle| \varepsilon_y\right)\right); -\infty < \varepsilon_y, \varepsilon_t < \infty,$$

where $P\left(r_y = k \middle| \varepsilon_y\right)$ is the same as $P(r_i = k|\tau_i)$ in Theorem 2. In order to obtain $P\left(\varepsilon_y \middle| \varepsilon_t\right)$, we need to know the conditional distribution of $\varepsilon_y$ given $\varepsilon_t$.

**Example:** Suppose the joint distribution of $\varepsilon_y$ and $\varepsilon_t$ is a Bivariate Normal, and the marginal distributions of $\varepsilon_y$ and $\varepsilon_d$ are univariate normal, i.e., $\varepsilon_y, \varepsilon_t \sim BVN(\mu_y, \mu_t, 1, 1, \rho)$ and $\varepsilon_y \sim N(\mu_y, 1)$ and $\varepsilon_t \sim N(\mu_t, 1)$, where $\mu_y$, $\mu_t$, and $\rho$ can be chosen arbitrarily. Then, the conditional distribution of $\varepsilon_y$ given $\varepsilon_t$ can be specified as $\varepsilon_y|\varepsilon_t \sim Normal\left(\mu_y + \rho(\varepsilon_t - \mu_t), 1 - \rho^2\right)$, which is a univariate normal distribution.

For simulation, we assumed that the joint distribution of $\varepsilon_y$ and $\varepsilon_t$ is a Bivariate Normal, and the marginal distributions of $\varepsilon_y$ and $\varepsilon_t$ are univariate normal, i.e., $\varepsilon_y,\ \varepsilon_t \sim BVN(0, 0, 1, 1, \rho)$ and $\varepsilon_y \sim N(0, 1)$ and $\varepsilon_t \sim N(0, 1)$, where the correlation coefficient, $\rho$, is chosen arbitrarily. Consequently, the conditional distribution of $\varepsilon_y$ given $\varepsilon_t$ is $\varepsilon_y|\varepsilon_t \sim Normal(\rho\varepsilon_t, 1 - \rho^2)$, which is a univariate normal distribution. Our goal is to observe the change of the relationship between the covariate and test statistics with the change of $\rho$. We would expect that the probability plots computed from test effect sizes are similar to the probability plots compute from the covariate effect sizes.

Figures 15.1-15.3 show the simulated relationship between the covariate effect and the test effect. To conduct the simulation, we adopted the importance sampling approach of the Monte Carlo simulation. As we see, in general, when the correlation is low ($\rho = .2$), the rank curves generated from the test effect (TH0 and TH1) are completely separated from the rank curves generated from the covariate effect (CH0 and CH1) and are quite flat in shape. As the correlation between effects increases, the test effect rank curves become more similar to the covariate rank curves and show a lot more variation with rank. Promisingly, at $\rho = 0.5$, the test effect curve tracks the covariate effect curve quite closely. This indicates that there does not have to be a high correlation between the two effect sizes in order for the method to be effective.

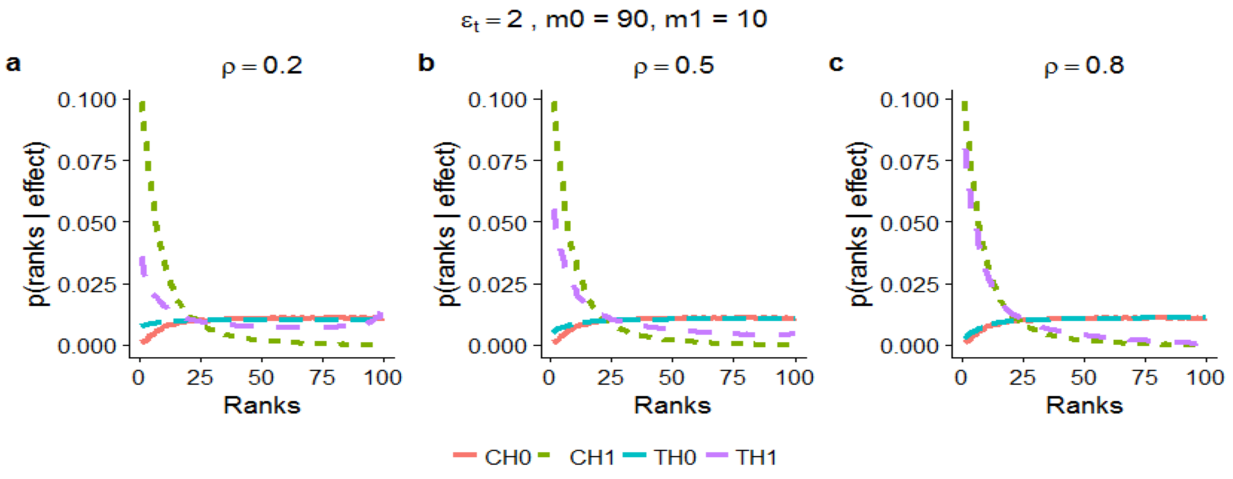


**Figure 15.1:** Relationship between the test effect (T) and the covariate effect (C) regarding the probability of the rank of test given the test effect size, $P(r_y = k|\varepsilon_t)$. In the legend, the first letter represents the source of the effects, and H0 and H1 represent the null and the alternative hypothesis, respectively. To generate the plots, we assumed that the number of hypothesis tests was $m = 100$, of which $m_0 = 90$ are true null and $m_1 = 10$ are true alternative tests; the test effect size of the alternative test is $\varepsilon_t = 2$; and the correlation varies by $\rho = \{.2, .5, .8\}$. We performed 10,000 replications to compute the probability of a specific rank, and for a specific rank, we generated 5,000 observations of $\tau_y$ from $Normal(\rho\varepsilon_t, 1-\rho^2)$ then computed the expectation of $P(r_y|\varepsilon_y)$ to obtain $P(r_y = k|\varepsilon_t)$.

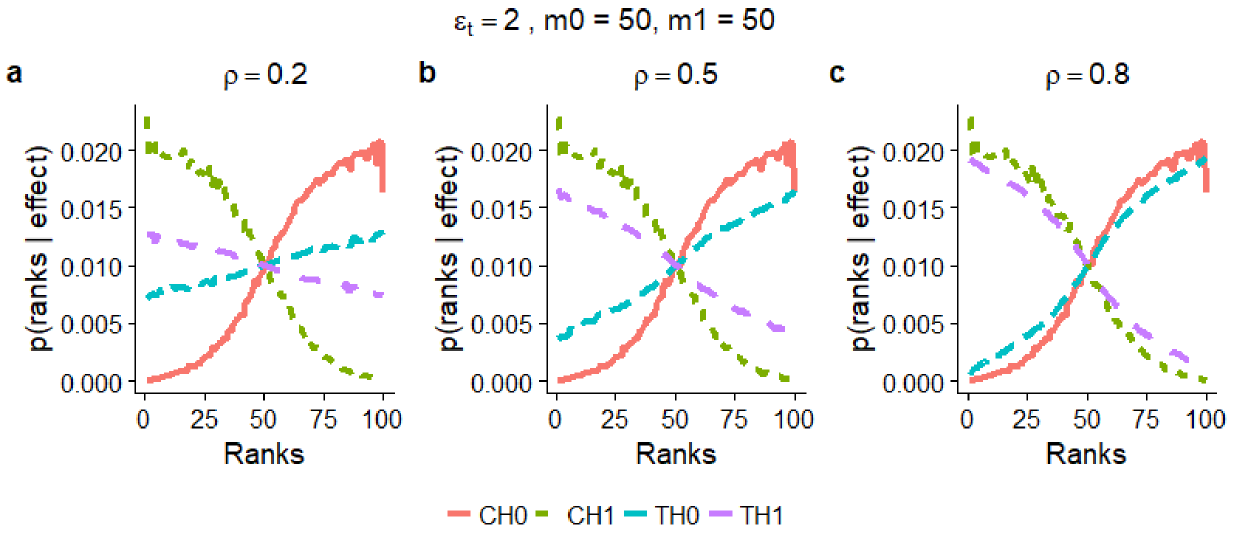


**Figure 15.2:** Relationship between the test effect (T) and the covariate effect (C). To generate the plots, we assumed that the number of hypothesis tests was $m = 100$, of which $m_0 = 50$ are true null and $m_1 = 50$ are true alternative tests; the mean test effect size of the alternative test is $\varepsilon_t = 2$; and the correlation varies by $\rho = \{.2, .5, .8\}$. We performed 10,000 replications to compute the probability of a specific rank, and for a specific rank, we generated 5,000

observations of $\varepsilon_y$ from $Normal(\rho\varepsilon_t,\ 1-\rho^2)$ then computed the expectation of $P(r_y|\varepsilon_y)$ to obtain $P(r_y = k|\varepsilon_t)$.

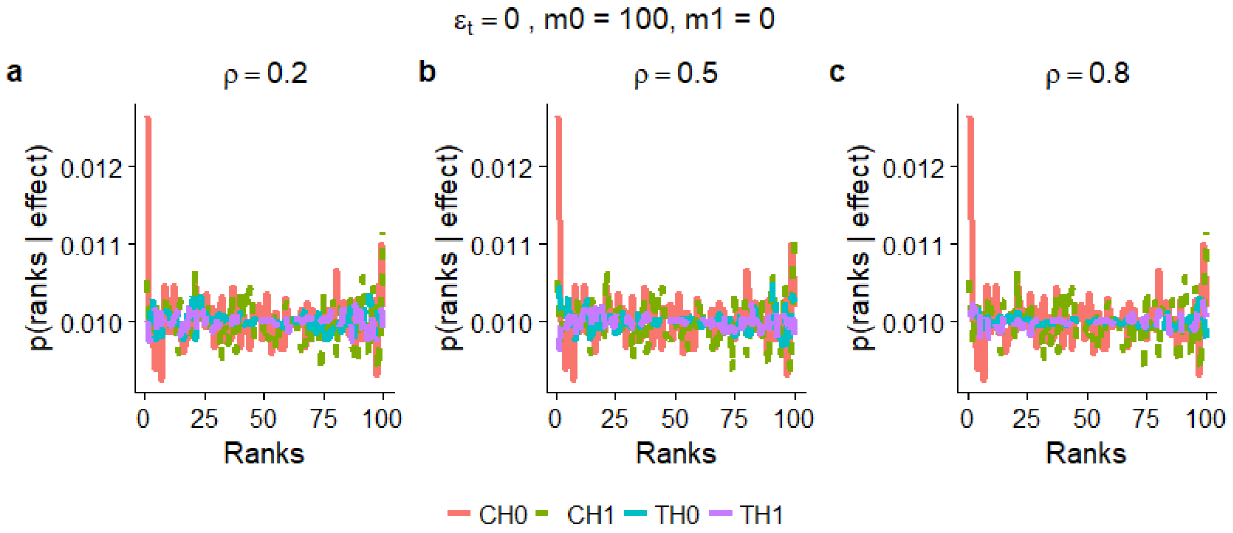


**Figure 15.3:** Relationship between the test effect (T) and the covariate effect (C). To generate the plots, we assumed that the number of hypothesis tests was $m = 100$, of which $m_0 = 100$ are true null and $m_1 = 0$ are true alternative tests; the mean test effect size is $\varepsilon_t = 0$; and the correlation varies by $\rho = \{.2,\ .5,\ .8\}$.

## 16. Nonlinear relationship between test effect and covariate effect

The weight formula (4) in the main text depends on the quantity $P(r_i|E(\varepsilon|\varepsilon > 0))$, where $r_i$ is the covariate rank for test $i$ and $\varepsilon$ is its effect size. That is, we need the covariate rank distribution for a test with effect size equal to the mean value among true alternative tests. We assume that there is a linear relationship between the test effect size $\varepsilon$ and the covariate effect size $\tau$. We conduct linear regression of estimated covariate effect sizes on estimated test effect sizes and use the fitted model to find the covariate effect that corresponds to the mean test effect.

In this section, we will consider what happens if the relationship between the two effect sizes is not linear. We assume that the covariate effect and test effect are related by

$$\tau = \frac{a\varepsilon}{1+\frac{\varepsilon}{b}} + N(0,\sigma^2)$$

This function is plotted without the noise term in Figure 16.1 below. The covariate effect has a saturating relationship with the test effect, increasing at a less than linear rate and flattening out as the test effect becomes large.

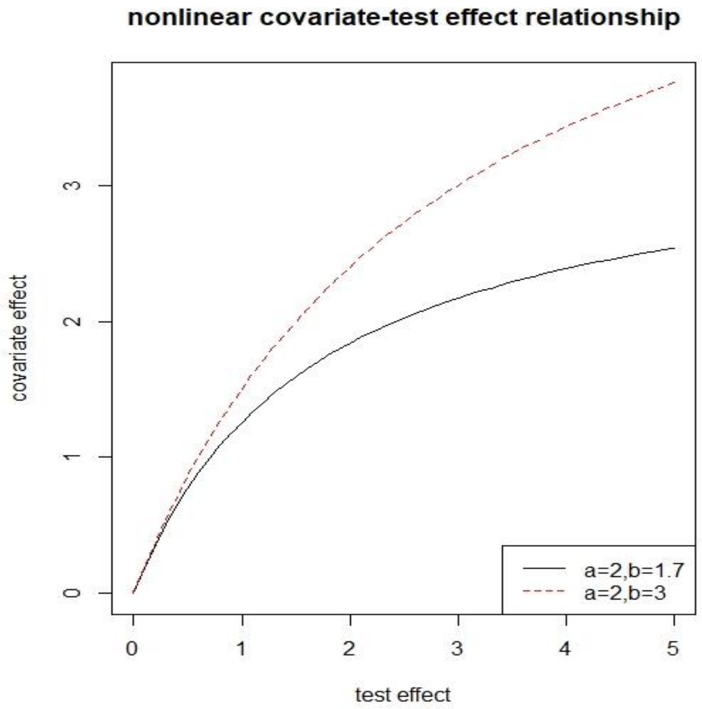


Figure 16.1 Nonlinear relationship between test and covariate effect.

We conducted simulations similar to those on the main text (see Section 4 above). The only difference is in how the simulated data were generated. The data were generated as follows:

1) Specify a mean test effect $e$
2) Generate a test effect vector $\vec{X}$ with each $X_i$ ~ uniform with mean of $e$.
3) Generate a covariate effect vector $\vec{Y} = \frac{a\vec{X}}{1+\frac{\vec{X}}{b}} + normal(0, \sigma^2)$

Figures 16.2 and 16.3 show power versus test effect size for CRW and three other methods with the relationship between covariate effect and test effect as shown in Figure 16.1. Figure 16.2 corresponds to the red dashed curve in Figure 16.1, while Figure 16.3 corresponds to the black solid curve. Power is decreased for the CRW method when there is a nonlinear relationship between test effect and covariate effect, although the effect is not large for the scenarios that we examined. The CRW is more affected than the IHW method. In most of the scenarios shown, the power is very similar between IHW and CRW. Thus, the relative advantage of CRW over IHW is lost, but there is no disadvantage to using CRW.

It would be straightforward to use nonlinear regression methods to model the relationship between test effect and covariate effect and thus the performance of CRW could be improved for the nonlinear case.

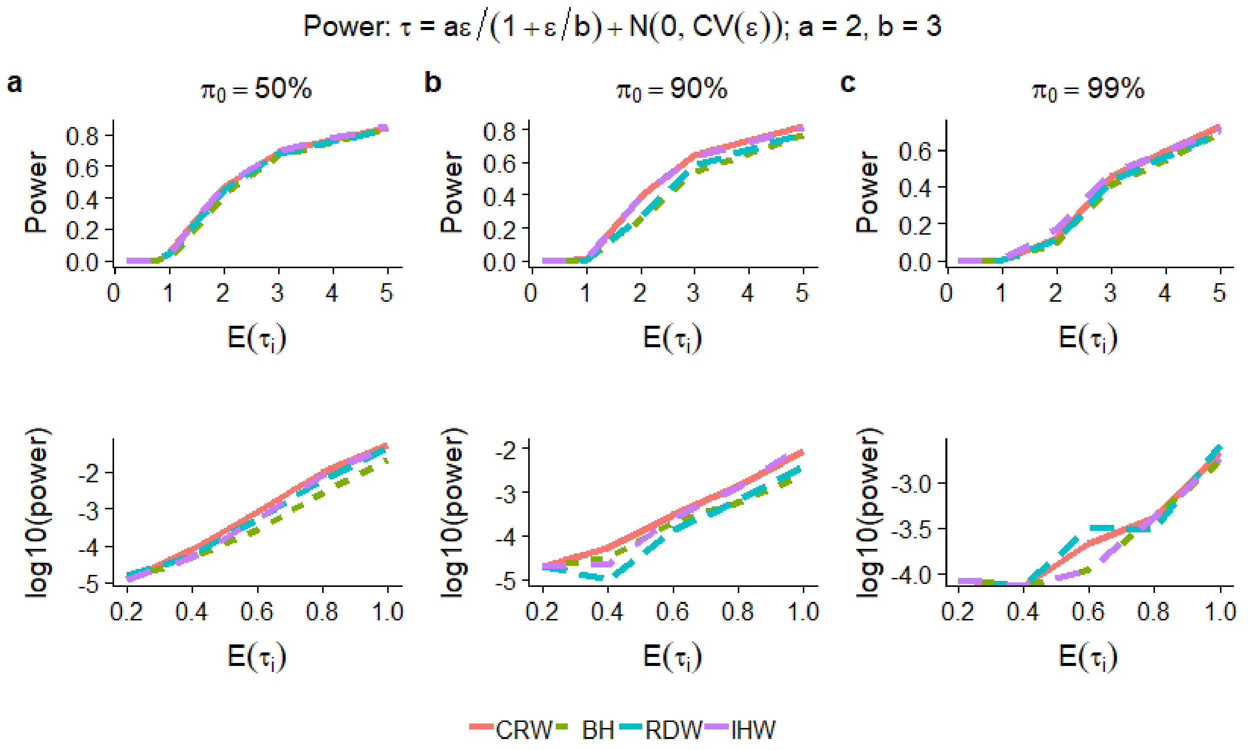


Figure 16.2: Power comparison between methods with nonlinear relationship between test and covariate effects.

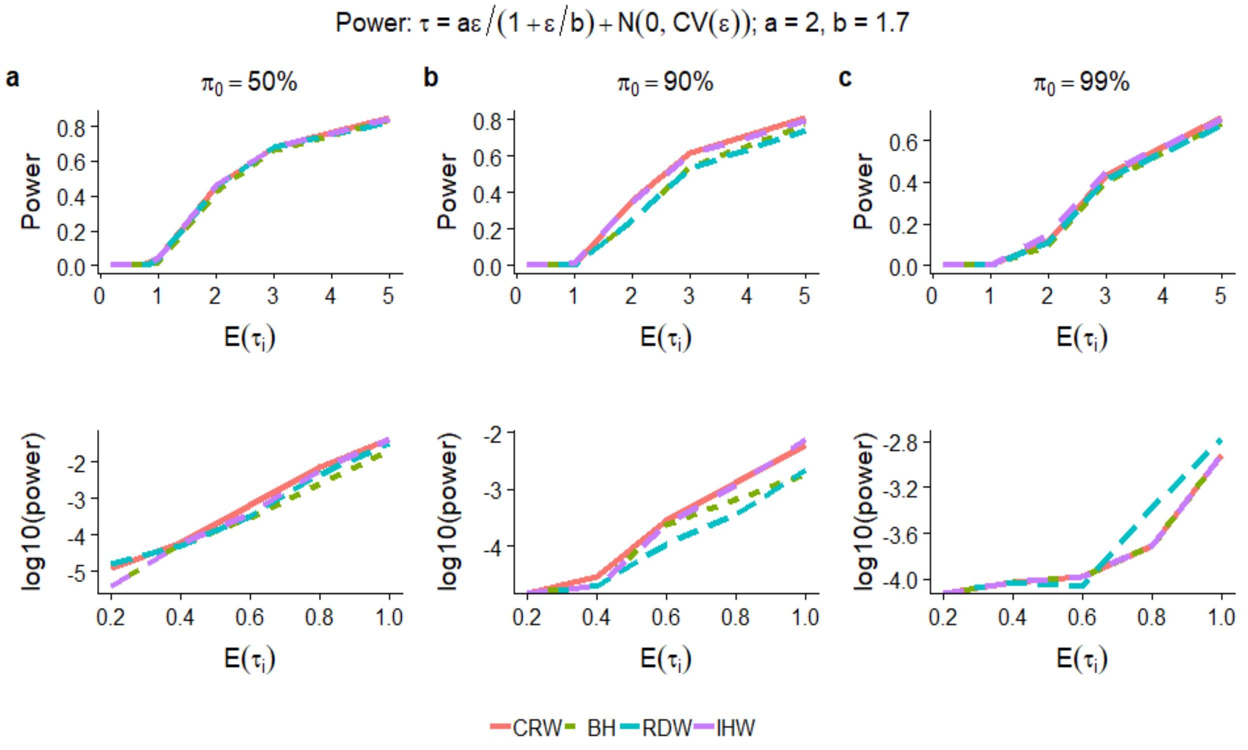


Figure 16.3: Power comparison between methods with nonlinear relationship between test and covariate effects.

## 17. Data Examples.

**Data source.** The CRW method was applied to the two data sets: Bottomly and Proteomics. *Bottomly* is discussed in Bottomly[3] and was downloaded from Recount project[8]. The authors generated single end RNA-Seq reads from *10 B6* and *11 D2* mice (21 lanes on three Illumina GAIIx flowcells). After applying the method described in the paper, the data had read counts for 36,229 genes of which 12,632 genes had no reads across all lanes, and 7,414 genes had no reads for at least one *B6* and one *D2* sample. Therefore, the subsequent analyses were based on the remaining 16,183 genes. We used *DESeq2* package[9] of Bioconductor to obtain the p-values and the mean of normalized counts (*baseMean*) for genes. We used *baseMean* for each gene across samples as the covariate.

*Proteomics* dataset is applied in the article[10]. The authors demonstrated an approach to increase the multiplexing capacity of quantitative mass spectrometry. By applying the approach, they quantified 2,666 proteins in six replicates. We used their Welch t-test p-values and the number of quantified peptides as the covariate from their supplementary Table 1.

We performed simple regression with Box-Cox transformation to obtain the relationship between the test and the covariate statistics in which covariate statistics were regressed on the test statistics. Then, by applying the model's information, we computed the predicted covariate statistics for the median and the mean test statistics. The predicted covariate statistics corresponding to the median and the mean were considered as the estimate of the covariate effect sizes. Note that, the diagnostic plots suggested that the models did not fit well. A Pin-point model diagnosis process can improve the fitness of the model. This leaves a scope of further research, which is beyond the goal of this article. However, the current model information is sufficient for our present purposes, because the CRW method only requires the centers of the test effect sizes and the corresponding covariate effect size.

### 17.1 Bottomly.

1) Covariate statistics is not normally distributed; therefore, we applied box-cox transformation in the simple linear regression.

2) Bimodal p-values indicate two-tailed test criteria are necessary because p-values close to 1 be the cases that are significant in the opposite direction.

3) Low p-values are enriched at high covariates or low ranks of the covariate statistics. This indicates that the covariate *baseMean* is correlated to the power under the alternative hypothesis test.

4) The empirical cumulative distribution shows whether the curve is almost linear for the high p-values.

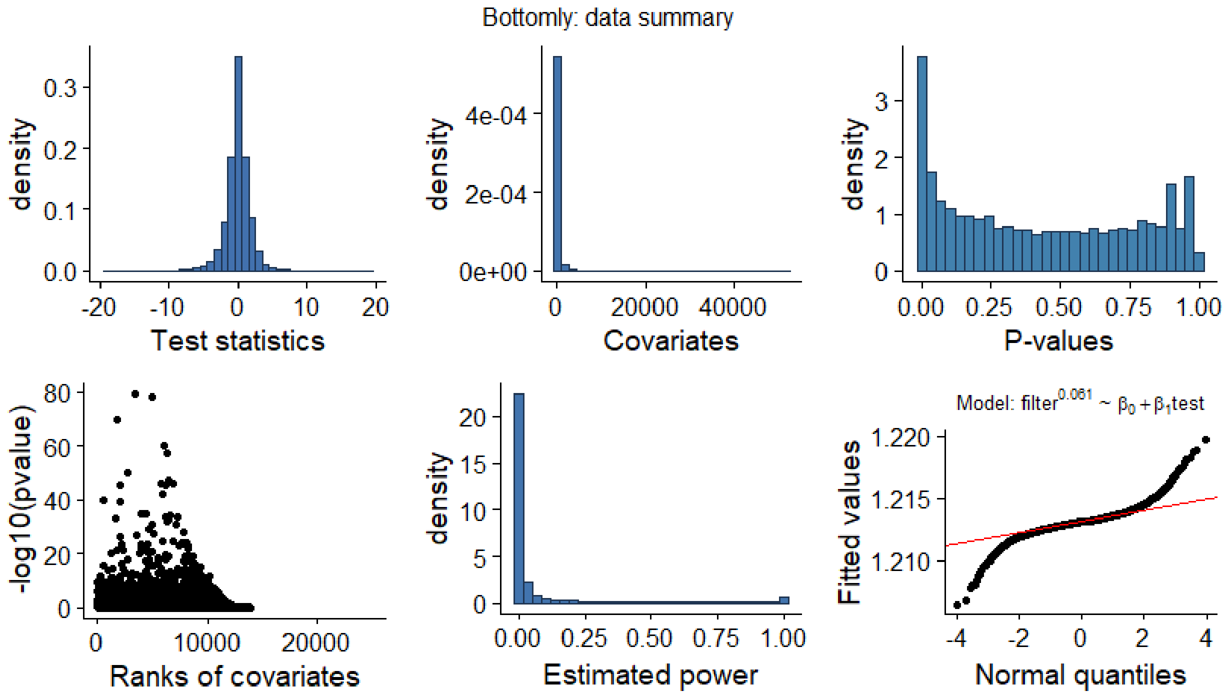


**Figure 17.1:** This Figure shows the summary information of the Bottomly-RNA-seq data. First row (left-right) shows the distribution of the test statistics, covariate statistics, and the p-values, respectively; and the second row shows the rank of the covariate statistics and the p-values (low index shows better rank), empirical cumulative distribution of the p-values, and the QQplot of the fitted values from the regression model with Box-Cox transformation.

**17.2 Proteomics.**

1) Covariate statistics is not normally distributed; therefore, we applied box-cox transformation in the simple linear regression.

2) Unimodal p-values indicate one-tailed test criteria are necessary.

3) There is a very weak relationship between high covariate values or low rank of the covariate statistics. This indicates that the covariate *peptide counts* is weakly correlated to the power under the alternative hypothesis test.

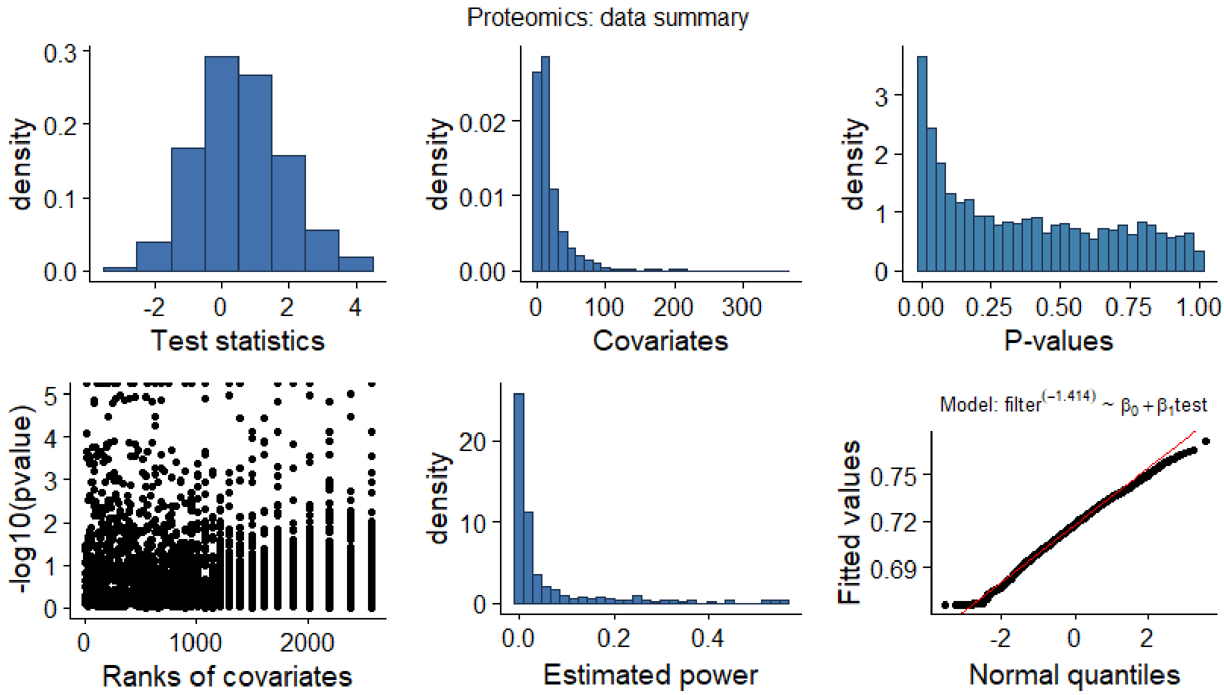


**Figure 17.2:** This Figure shows the summary information of the Proteomics data. First row (left-right) shows the distribution of the test statistics, covariate statistics, and the p-values, respectively; and the second row shows the rank of the covariate statistics and the p-values (low index shows better rank), empirical cumulative distribution of the p-values, and the QQ plot of the fitted values from the regression model with Box-Cox transformation.

**18. Approximate vs. exact weights.**

For the comparative study, we computed the exact weights via solving the integration of the objective problem numerically (Equation 5 in the original article) and compared with the approximate weights that we proposed called CRW (Theorem 1). We applied the exact and the approximate procedures on the two data sets.

To apply the exact method, we transformed the covariates by Box-Cox transformation since covariates are not approximately normal. Then, we estimated the true alternative mean and the standard deviation to compute the ranks probability and the corresponding weights. In this procedure, we assumed that the transformed covariates are normally distributed. On the other hand, to compute the approximate weights, we followed the data analysis steps described in the online methods (data examples section).

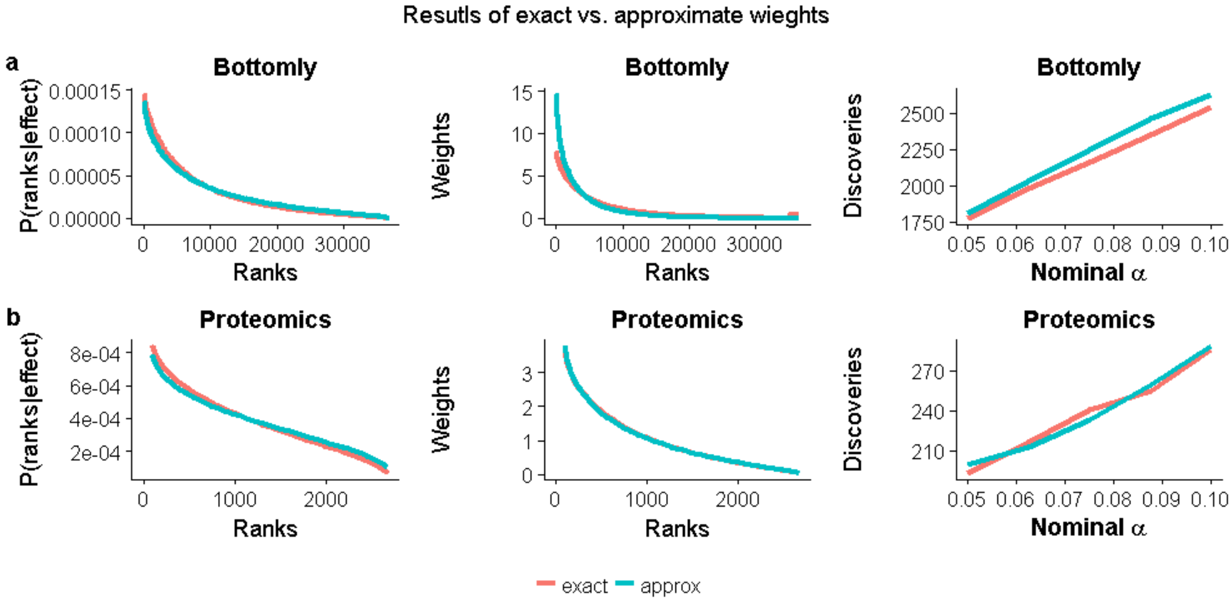


**Figure – 18.1:** This Figure shows the comparison between the exact and the approximate weights and the corresponding results. a) Results of the Bottomly data: ranks probability, weights at $\alpha = .05$, and the number of rejected tests at the different significance level of $\alpha$. b) Results of the Proteomics data: ranks probability, weights at $\alpha = .05$, and the number of rejected tests at the different significance level of $\alpha$.

## 19. Algorithm to compute CRW weights

To obtain the optimal value of $\delta$, we applied Newton-Raphson and Grid search algorithms. Let us denote a function of $\delta$ by $f(\delta)$, then applying the weighting constraint $\frac{1}{m}\sum_{i=1}^{m} w_i = 1$, we have

$$f(\delta) = \sum_{i=1}^{m} \left(\frac{m}{\alpha}\right) \bar{\Phi} \left( \frac{E(\varepsilon)}{2} + \frac{1}{E(\varepsilon)} log \left( \frac{\delta}{\alpha P\left(r_i \middle| E(\varepsilon)\right)} \right) \right) - \alpha \ldots \ldots \ldots . (19.1)$$

We solved $f(\delta)$ for $\delta \epsilon [0, \infty)$. Generally, we applied the Newton-Raphson (NR) algorithm to obtain the optimal value of $\delta$ when $f(\delta) > 0$. Although NR is computationally faster, it heavily depends on the correct guess of the initial value. NR method is also sensitive to non-convex problem. From the simulation results, it is evident that if the effect size is very low, we will have flatter weights, then NR method does not converge and unable to find the roots. Therefore, we used grid search algorithm for $\delta \epsilon [0, 1)$ and NR for $\delta \epsilon (1, \infty)$ to obtain the optimal value of $\delta$.

See next page for the algorithm.

**Algorithm: Compute CRW weights**

---

**Input:** $m \leftarrow$ total number of hypothesis tests; $\alpha \in (0, 1) \leftarrow$ significance threshold;

$E(\varepsilon) \leftarrow$ mean of test-effect; $P(r_i \mid E(\tau)) \leftarrow$ ranks probabilities

$f \leftarrow$ function of $\delta$ from equation (19.1)

$f' \leftarrow$ first derivative of $f$

Denote $nmax = 100$ and let an initial value $x_0$

$n = 1$

***if*** $(\boldsymbol{n} <= \boldsymbol{nmax}))$ ***then***

***while*** $(\boldsymbol{f}(\boldsymbol{x0}) < \boldsymbol{0})$ ***do***

***if*** $(\boldsymbol{f}(\boldsymbol{x_0} + \boldsymbol{0}) > \boldsymbol{f}(\boldsymbol{x_0} + .\boldsymbol{5}))$ ***then***

$x_0 = x_0 - .5$

***else***

$x_0 = x_0 + .5$

***end***

$n = n + 1$

***end***

solve $f(\delta)$ for $\delta \in [0, \infty)$ using Newton-Raphson method and return $\delta_{opt}$

***else***

Generate a sequence of $\delta = \delta_1, \ldots, \delta_n$, where $\delta \in (0,1)$ and

$|\delta_j - \delta_k| \leq .001;\ j, k = 1, \ldots, n; j \neq k.$

For each $\delta_j$, compute the sum of weights $sw_j(\delta_j) = \sum_{i=1}^{m} w_i$ via Theorem 1

Denote by $\delta_{opt}$ the optimal value of $\delta$, which satisfy $\min_{\delta_{opt}} |sw_j(\delta_j) - m|$

***end***

Compute the weights $w$ by using $\delta_{opt}$

Normalize the weights $\overline{w}$ so that the weights sum to $m$

***Return:*** $w, \delta_{opt}$

---

**References**


1. Storey, J. D. & Tibshirani, R. Statistical significance for genomewide studies. *Proc. Natl. Acad. Sci. U. S. A.* **100,** 9440–9445 (2003).

2. Efron, B. Size, power, and false discovery rates. *Ann. Stat.* **35,** 1351–1377 (2007).

3. Bottomly, D. *et al.* Evaluating gene expression in C57BL/6J and DBA/2J mouse striatum using RNA-Seq and microarrays. *PLoS One* **6,** e17820 (2011).

4. Benjamini, Y. & Hochberg, Y. Multiple hypotheses testing with weights. *Scand. J. Stat.* **24,** 407–418 (1997).

5. Roeder, K. & Wasserman, L. Genome-Wide Significance Levels and Weighted Hypothesis Testing. *Stat. Sci.* **24,** 398–413 (2009).

6. Ignatiadis, N., Klaus, B., Zaugg, J. & Huber, W. Data-driven hypothesis weighting increases detection power in big data analytics. *bioRxiv* **13,** 034330 (2015).

7. Wasserman, L., Roeder, K. & Laan, V. Der. Weighted Hypothesis Testing. (2006).

8. Frazee, A. C., Langmead, B. & Leek, J. T. ReCount: A multi-experiment resource of analysis-ready RNA-seq gene count datasets. *BMC Bioinformatics* **12,** 449 (2011).

9. Love, M. I., Huber, W. & Anders, S. Moderated estimation of fold change and dispersion for RNA-seq data with DESeq2. *Genome Biol.* **15,** 550 (2014).

10. Dephoure, N. & Gygi, S. P. Response to Rapamycin in Yeast. **5,** 1–16 (2017).
